# Supplementary material for: A Drug Recommendation System (Dr.S) for cancer cell lines
Source: arXiv:1912.11548 ancillary file (2019-12-24)
Supplement: Supplementary file 1 [file supportingInfo.pdf]

# Supporting Information: A Drug Recommendation System (Dr.S) for cancer cell lines

Marleen Balvert[1,2], Georgios Patoulidis[3], Andrew Patti[3], Timo M. Deist[4], Christine Eyler[3], Bas E. Dutilh[2], Alexander Schönhuth[1,2], and David Craft[3]

[1] *Life Sciences & Health, Centrum Wiskunde & Informatica, Amsterdam, 1098 XG, The Netherlands*

[2] *Theoretical Biology & Bioinformatics, Utrecht University, Utrecht, 3512 JE, The Netherlands*

[3] *Massachusetts General Hospital and Harvard Medical School, Department of Radiation Oncology, Boston MA*

[4] *The D-Lab, Dpt of Precision Medicine, GROW - School for Oncology and Developmental Biology, Maastricht University Medical Centre+, Maastricht, The Netherlands*

December 24, 2019

## 1 Gene set combos

Assume we have a set of gene sets $L_i$, i=[0,1,2, .. H]. Gene set $L_0$ is the empty set, $L_i$, $i = 1, 2, \ldots H$ are proper gene subsets, for example the radiation gene set. Also note that if we want to include gene sets that are unions or intersections of more primitive gene sets, e.g. if we wanted to put the radiation gene set and another set together, we would do this explicitly and include that combined gene set in the set set L (i.e. we do not write code to do it automatically).

Assume we also have G different types of gene level data: for example, G might equal 3: gene expression, mutation, and copy number data. We then will make every possible run for these subsets. Let ie be the index for gene expression, im the index for gene mutation, and ic the index for copy number.

**Algorithm 1:** Form set of all combos $C$

```
Initialize C = {};
foreach gene expression index ie ∈ 0...H do
    foreach gene mutation index im ∈ 0...H do
        foreach gene copy number index ic ∈ 0...H do
            if ie == 0 & im == 0 & ic == 0 then
                continue
            else
                Expression gene set = L_ie
                Expression gene set = L_ie
                Expression gene set = L_ie

                store combo c = {Expression gene set, Mutation gene set, and Copy Number
                  gene set } in set C
            end
        end
    end
end
```

## 2 Double data split strategy in pseudo-code

**Algorithm 2:** Double split looping for CLA MAS module

```
foreach algorithm a ∈ A do
    foreach combo c ∈ C do
        for outer MCCV repetition i = 1 : 10 do
            randomly sample 80% of all rows (cell lines) as outer-training data;
            assign the remaining rows as outer-holdout data;
            for inner MCCV repetition j = 1 : 10 do
                randomly subsample 80% of all outer-training rows as inner-training data;
                assign the remaining rows as inner-holdout data;
                foreach hyperparameter configuration h_a ∈ H_a do
                    train algorithm a with hyperparameter configuration h_a on inner-training
                      data;
                    predict outcomes for inner-holdout data;
                    compute performance metric p_{c,a,h_a,j} on inner-holdout data predictions;
                end
            end
            compute p_{c,a,h_a}, the average of the 10 performance metrics p_{c,a,h_a,j} for each
              hyperparameter configuration h_a;
            select hyperparameter configuration h*_a with best average inner-holdout
              performance metric p_{c,a,h_a};
            train algorithm a with hyperparameter configuration h*_a on outer-training data;
            predict outcomes for outer-holdout data;
            compute performance metric P_{c,a,i} on outer-holdout data predictions;
        end
        compute P_{c,a}, the average of the 10 performance metrics P_{c,a,i};
    end
end
compare P_{c,a}
```

$A$ is the set of algorithms $a$: random forest, linear SVM, RBF SVM, etc.

$H_a$ is the set of possible hyperparameters combinations $h_a$ for algorithm $a$.

MCCV is Monte-Carlo Cross Validation

# 3 Hyperparameter tuning

| Algorithm | Hyperparameter | Candidates |
|---|---|---|
| Random Forest | max_features | $\sqrt{p}$, $(\sqrt{p}+p)/2)$, $p$ |
| Random Forest | min_samples_split | 2, 10, 20 |
| Elastic Net | alpha | 0.01, 0.1, 1, 10 |
| Elastic Net | l_one_ratio | 0, 0.1, 0.5, 0.9, 1.0 |
| Radial Basis Function SVM | c | 0.01, 0.1, 1 |
| Radial Basis Function SVM | gamma | $10^{-5}$, $10^{-4}$, $10^{-3}$, 0.01, 0.1, 1, 10 |

Table 1: Hyperparameters and their values available for each algorithm. $p$ is number of features.

# 4 Gene sets

The Cosmic (Catalog of Somatic Mutations in Cancer) gene set contains curated genes from the Sanger initiative. Gene set MAPK contains genes in that pathway from biocarta, see `http://software.broadinstitute.org/gsea/msigdb/cards/BIOCARTA_MAPK_PATHWAY`. Gene set Rhodes contains genes upregulated in cancer cells Rhodes et al. [2004]. Gene set Radiation is our custom curated set for the genes thought to be most important for the fate of a cell after radiation damage, see Section 4.2. Gene set sigcancer is a set of genes useful for identifying tumor tissue origin Xu et al. [2016]. Gene set general is manually curated from two text books identifying genes generally important for cancer Graw [2015], Schmidt [2017]. The genes in each gene set are given below.

Table 2: Genes included in gene set Cosmic.

| | | | | | | | |
|---|---|---|---|---|---|---|---|
| ABL1 | ACVR1 | ACVR1B | ACVR2A | AKT1 | ALK | AMER1 | APC |
| AR | ARID1A | ARID2 | ASXL1 | ATM | ATP1A1 | ATP2B3 | ATR |
| ATRX | AXIN1 | AXIN2 | BAP1 | BCL9L | BCOR | BIRC3 | BRAF |
| BRCA1 | BRCA2 | BTK | CACNA1D | CALR | CARD11 | CASP8 | CBL |
| CBLB | CD79A | CD79B | CDC73 | CDH1 | CDKN2A | CDKN2C | CEBPA |
| CIC | CNOT3 | COL2A1 | CREBBP | CRLF2 | CSF1R | CSF3R | CTNNA1 |
| CTNNB1 | CUX1 | CXCR4 | CYLD | DAXX | DDR2 | DGCR8 | DICER1 |
| DNM2 | DNMT3A | DROSHA | EGFR | EML4 | EP300 | EPAS1 | ERBB2 |
| ERBB3 | ERBB4 | ERG | ESR1 | ETNK1 | EZH2 | FAT1 | FAT4 |
| FBXO11 | FBXW7 | FGFR1 | FGFR2 | FGFR3 | FLT3 | FOXA1 | FOXL2 |
| FUBP1 | GATA1 | GATA2 | GATA3 | GNA11 | GNAQ | GNAS | GRIN2A |
| H3F3A | H3F3B | HIF1A | HIST1H3B | HNF1A | HRAS | IDH1 | IDH2 |
| IKBKB | IKZF1 | IL6ST | IL7R | JAK1 | JAK2 | JAK3 | KCNJ5 |
| KDM5C | KDM6A | KDR | KEAP1 | KIT | KLF4 | KMT2C | KMT2D |
| KRAS | LRP1B | LZTR1 | MAP2K1 | MAP2K2 | MAP2K4 | MAP3K13 | MAX |
| MED12 | MEN1 | MET | MLH1 | MPL | MSH2 | MSH6 | MTOR |
| MYD88 | MYOD1 | NCOA2 | NCOR1 | NF1 | NF2 | NFE2L2 | NFKBIE |
| NOTCH1 | NOTCH2 | NPM1 | NRAS | NT5C2 | NTRK3 | PAX5 | PBRM1 |
| PDGFRA | PHF6 | PHOX2B | PIK3CA | PIK3R1 | PLCG1 | POLD1 | POLE |
| POT1 | PPM1D | PPP2R1A | PPP6C | PRDM1 | PREX2 | PRKACA | PRKAR1A |
| PTCH1 | PTEN | PTK6 | PTPN11 | PTPN13 | PTPRB | RAC1 | RAD21 |
| RB1 | RET | RHOA | RNF43 | RPL10 | RPL5 | RUNX1 | SETBP1 |
| SETD2 | SF3B1 | SH2B3 | SIX1 | SIX2 | SMAD2 | SMAD3 | SMAD4 |
| SMARCA4 | SMARCB1 | SMARCD1 | SMO | SOCS1 | SPEN | SPOP | SRC |
| SRSF2 | STAG2 | STAT3 | STAT5B | STK11 | SUFU | TBL1XR1 | TBX3 |
| TERT | TET2 | TGFBR2 | TNFAIP3 | TNFRSF14 | TP53 | TP63 | TRAF7 |
| TSC1 | TSC2 | TSHR | U2AF1 | UBR5 | USP8 | VHL | WT1 |
| XPO1 | ZFHX3 | ZRSR2 | FAM123B | MLL2 | MLL3 | | |

Table 3: Genes included in gene set general.

| | | | | | | | |
|---|---|---|---|---|---|---|---|
| ACD | APAF1 | ARNT | ATG5 | ATM | BAD | BAK1 | BAX |
| BCL2 | BCL2A1 | BCL2L1 | BCL2L2 | BRAF | BRCA1 | BRCA2 | BUB3 |
| CASP3 | CASP7 | CASP8 | CASP9 | CCND1 | CCND2 | CDK4 | CDKN2A |
| CFLAR | CTNNB1 | CYC1 | CYCS | E2F1 | E2F2 | E2F3 | E2F4 |
| E2F5 | E2F6 | E2F7 | E2F8 | EGFR | ERBB2 | FADD | FASLG |
| FGF1 | FGF2 | FGFR4 | FH | FLT1 | FLT4 | GLUL | HRAS |
| IGF1R | IGF2 | KDR | KIT | KRAS | MAD1L1 | MAD2L1 | MCL1 |
| MDM2 | MET | MLKL | MXD3 | MYC | MYCL | MYCN | NF1 |
| NF2 | NOX1 | NRAS | PCSK1 | PIGF | PKM | PYGL | RAP1A |
| RB1 | RELA | RET | RIPK1 | RIPK3 | SH2B2 | SKP2 | SLC16A1 |
| SLC2A1 | SMO | SNAI2 | TAL1 | TERF1 | TERF2 | TGFA | TINF2 |
| TNFSF10 | TP53 | TPP1 | TRADD | VEGFB | WNT1 | WT1 | ZEB2 |
| MYCL1 | PKM2 | | | | | | |

Table 4: Genes included in gene set MAPK.

| | | | | | |
|---|---|---|---|---|---|
| ARAF | ATF2 | BRAF | CEBPA | CHUK | CREB1 |
| DAXX | ELK1 | FOS | GRB2 | HRAS | IKBKB |
| JUN | MAP2K1 | MAP2K2 | MAP2K3 | MAP2K4 | MAP2K5 |
| MAP2K6 | MAP2K7 | MAP3K1 | MAP3K10 | MAP3K11 | MAP3K12 |
| MAP3K13 | MAP3K14 | MAP3K2 | MAP3K3 | MAP3K4 | MAP3K5 |
| MAP3K6 | MAP3K7 | MAP3K8 | MAP3K9 | MAP4K1 | MAP4K2 |
| MAP4K3 | MAP4K4 | MAP4K5 | MAPK1 | MAPK10 | MAPK11 |
| MAPK12 | MAPK13 | MAPK14 | MAPK3 | MAPK4 | MAPK6 |
| MAPK7 | MAPK8 | MAPK9 | MAPKAPK2 | MAPKAPK3 | MAPKAPK5 |
| MAX | MEF2A | MEF2BNB-MEF2B | MEF2C | MEF2D | MKNK1 |
| MKNK2 | MYC | NFKB1 | NFKBIA | PAK1 | PAK2 |
| RAC1 | RAF1 | RAPGEF2 | RELA | RIPK1 | RPS6KA1 |
| RPS6KA2 | RPS6KA3 | RPS6KA4 | RPS6KA5 | RPS6KB1 | RPS6KB2 |
| SHC1 | SP1 | STAT1 | TGFB1 | TGFB2 | TGFB3 |
| TGFBR1 | TRADD | TRAF2 | | | |

Table 5: Genes included in gene set radiation.

| | | | | | |
|---|---|---|---|---|---|
| ABL1 | AKT1 | ALK | APAF1 | APC | AR |
| ATM | ATP13A1 | ATP13A2 | ATP2C1 | ATP2C2 | ATR |
| AURKA | AURKB | AURKC | BAD | BAP1 | BAX |
| BBC3 | BCL2 | BCL2L1 | BCL2L11 | BECN1 | BID |
| BIRC2 | BIRC3 | BIRC5 | BLM | BMI1 | BMPR1A |
| BMPR1B | BMPR2 | BRAF | BRCA1 | BRCA2 | BRIP1 |
| BUB1 | CAT | CCNB1 | CCND1 | CCND3 | CDC25C |
| CDH1 | CDK1 | CDK2 | CDK4 | CDK6 | CDKN1A |
| CDKN1B | CDKN2A | CDKN2A-DT | CDKN2B | CHEK1 | CHEK2 |
| CNNM1 | CREB1 | CTNNB1 | DCLRE1C | DDB2 | DKC1 |
| DLX2 | DNM1 | DRAM1 | E2F1 | EGFR | EP300 |
| EPAS1 | ERBB2 | ERCC5 | ERCC6 | ESR1 | EXO1 |
| FADD | FANCD2 | FAS | FGFR1 | FGFR2 | FGFR3 |
| FN1 | FZD1 | G6PD | GABPA | GABPB1 | GABPB2 |
| GADD45A | GJA1 | GJB1 | GJB2 | GLI1 | GLS |
| GLUD1 | GOT1 | GRB2 | GSX1 | GSX2 | H2AFX |
| HDAC1 | HIF1A | HIPK2 | HIST1H2BC | HRAS | HSP90AA1 |
| IDH1 | IDH2 | IGFBP3 | IL6 | IL6R | IL6ST |
| INSR | IRF1 | JAK1 | JAK2 | JUN | KLF4 |
| KMT2C | KRAS | LEF1 | LIG4 | LSP1 | MAP1LC3A |
| MAP2K7 | MAPK1 | MAPK14 | MAPK3 | MAPK8 | MAX |
| MDC1 | MDM2 | MGMT | MLH1 | MRE11 | MSH2 |
| MSH3 | MSH6 | MTOR | MYC | MYCN | NBN |
| NCOA4 | NEDD4L | NFKB1 | NFKB2 | NHEJ1 | NOS1 |
| NOS2 | NOS3 | NOTCH1 | NOTCH2 | NOTCH3 | NOTCH4 |
| NRAS | P2RX4 | PALB2 | PARP1 | PARP2 | PGAP3 |
| PGR | PIK3CA | PIK3CB | PLK1 | PLK2 | PLK3 |
| PMAIP1 | PPM1D | PRDX1 | PRDX2 | PRDX4 | PRDX6 |
| PRKCA | PRKCB | PRKCD | PRKDC | PSENEN | PTCH1 |
| PTEN | PTGS2 | RAD18 | RAD50 | RAD51 | RARA |
| RB1 | RBBP8 | RECQL4 | RELA | RIF1 | RIPK1 |
| RNF168 | RPRM | RTEL1 | SDHA | SDHB | SERPINE1 |
| SFN | SHH | SIAH1 | SIAH2 | SLC11A1 | SLC11A2 |
| SLC25A39 | SLC30A10 | SLC31A1 | SLC34A2 | SLC34A3 | SLC36A1 |
| SLC39A14 | SLC39A8 | SLC6A3 | SMAD2 | SMAD3 | SMAD4 |
| SMO | SNAI1 | SNRPF | SOD1 | SOD2 | SOD3 |
| SOX2 | SPARC | STAT1 | STAT3 | SUMO1 | TCF7 |
| TERC | TERT | TET1 | TGFB1 | TGFBR1 | TGFBR2 |
| THBS1 | TLR9 | TNF | TNFAIP3 | TNFRSF10B | TNFRSF13B |
| TNFRSF1A | TNFRSF1B | TOPBP1 | TOX3 | TP53 | TP53BP1 |
| TSC1 | TSC2 | TXNIP | UIMC1 | VDR | VIM |
| WEE1 | WNT3A | WNT5A | WNT7A | WRN | WT1 |
| XIAP | XPC | XRCC4 | XRCC5 | XRCC6 | XYLT2 |
| YWHAQ | YWHAZ | ZEB1 | ZHX2 | MRE11A | |

Table 6: Genes included in gene set rhodes.

| | | | | | | | |
|---|---|---|---|---|---|---|---|
| ACLY | AHCY | CANX | CBX3 | CCT4 | CCT5 | CDK1 | CDKN3 |
| CKS2 | COL1A2 | COPB2 | CRIP2 | DVL3 | E2F5 | EIF4A3 | FAP |
| G3BP1 | HDAC1 | HNRNPA2B1 | HSPD1 | HSPE1 | IARS | IFNGR2 | ILF2 |
| KDELR2 | KIAA0101 | KPNA2 | LDHA | MANF | MCM3 | MMP9 | MRPL3 |
| MRPS12 | MTHFD2 | NCBP2 | NME1 | NONO | NUP205 | OGT | PAFAH1B3 |
| PAICS | PLK1 | PPP2R5C | PRDX4 | PSMC4 | PSME2 | PTMA | RBM4 |
| RFC4 | SDHC | SMARCA4 | SNRPE | SNRPF | SOX4 | SSBP1 | SSR1 |
| TARS | TGIF1 | TOP2A | TPX2 | TRAF4 | TSTA3 | TUBB | UBE2S |
| PCLAF | | | | | | | |

Table 7: Genes included in gene set sigcancer.

| | | | | | |
|---|---|---|---|---|---|
| ACPP | ACTC1 | ACTG2 | AGR2 | ALDH1A2 | APOBEC3B |
| APOD | ASPN | ATP1B1 | AZGP1 | C4BPA | C7 |
| CA12 | CALB2 | CARTPT | CCL18 | CDH1 | CDH17 |
| CEACAM5 | CEACAM6 | CHGA | CHGB | CHI3L1 | CHRNA3 |
| CKB | CLDN11 | CLDN18 | CLU | COL11A1 | CPB1 |
| CXCL14 | CXCL5 | CYP17A1 | DBH | DCT | DDX3Y |
| DLK1 | DMBT1 | EFEMP1 | EGFL6 | EGFR | EPCAM |
| ESR1 | FABP1 | FABP4 | FAM107A | FOXE1 | GATA3 |
| GCG | GFAP | GJA1 | GPM6B | GPX3 | GREM1 |
| HBB | HLA-DQA1 | ID4 | IGFBP2 | IGFBP7 | IGJ |
| INSM1 | ISL1 | KCNJ16 | KLK2 | KLK3 | KRT1 |
| KRT13 | KRT14 | KRT15 | KRT19 | KRT20 | KRT4 |
| KRT7 | L1TD1 | LGALS4 | LIPF | LUM | MAB21L2 |
| MGP | MITF | MLANA | MMP1 | MMP12 | MMP3 |
| MS4A1 | MSLN | MSMB | MSX1 | MT3 | NKX2-1 |
| NKX3-1 | NPTX2 | NPY1R | OGN | OR51E2 | PAPPA |
| PAX3 | PCDH7 | PCP4 | PEG3 | PHOX2B | PI15 |
| PIGR | PIP | PLA2G2A | POSTN | POU3F3 | PRRX1 |
| PTGDS | PTN | PTX3 | RGS4 | RPS11 | RPS4Y1 |
| S100A2 | S100A8 | S100P | SCG5 | SCGB1A1 | SCGB2A2 |
| SERPINA3 | SERPINA5 | SERPINB3 | SERPINB4 | SFN | SFRP1 |
| SFTPB | SFTPC | SFTPD | SLC26A3 | SLC26A4 | SLC2A3 |
| SLC3A1 | SPINK1 | SPP1 | SST | STAR | SULT2A1 |
| TACSTD2 | TG | TH | THBS4 | TM4SF4 | TPO |
| TRPM1 | TRPS1 | TSHR | TSPAN8 | TSPYL5 | TTR |
| TYR | TYRP1 | VEGFA | XIST | JCHAIN | |

### 4.1 Gene set overlap

| | **cosmic** | **MAPK** | **general** | **radiation** | **rhodes** | **sigcancer** |
|---|---|---|---|---|---|---|
| **cosmic** | *222* | 11 | 22 | 58 | 1 | 6 |
| **MAPK** | 11 | *87* | 6 | 18 | 0 | 0 |
| **general** | 22 | 6 | *98* | 29 | 1 | 1 |
| **radiation** | 58 | 18 | 29 | *263* | 5 | 5 |
| **rhodes** | 1 | 0 | 1 | 5 | *65* | 0 |
| **sigcancer** | 6 | 0 | 1 | 5 | 0 | *155* |

Table 8: Gene set overlap. Number of genes in each set is on the diagonal. The off-diagonal entries are the number of genes in common between the column and the row gene sets. The union of the sets contains 754 unique genes.

## 4.2 Creation of the Radiation gene set

A hybrid approach utilizing expert-based and citation-based selection and prioritization of likely genes associated with radiation response was performed using a scoring system incorporating both elements, with the top overall scoring genes being retained in the final gene set. Three independent internal experts/groups generated gene sets thought to represent genes likely to represent radiation modulators; genes were scored based on their inclusion in each set (i.e., if appearing in only one set a gene received a score of one, if in two sets a score of two, if in all three sets a score of three for this criterion). A fourth set was generated using an objective citation-based prioritization via NCBI's PubMed using the following search:

"(Radiation Tolerance*[Mesh] OR Radiation, Ionizing* [Mesh] OR Radiation-Protective Agents*[Mesh] OR Cell Death/radiation effects*[Mesh] OR Apoptosis/radiation effects*[Mesh] OR dna damage/ radiation effects*[Mesh Terms] OR Cellular Senescence/radiation effects*[Mesh] OR Chromosome Aberrations/radiation effects*[Mesh] OR Bystander Effect/radiation effects*[Mesh] OR Autophagy/ radiation effects*[Mesh] OR Cell Cycle/radiation effects*[Mesh] OR Reactive Oxygen Species/ radiation effects*[Mesh] OR Oxidative Stress/radiation effects*[Mesh] OR Metabolism/radiation effects* [Mesh] OR Transcription, Genetic/radiation effects*[Mesh] OR Stem Cells/radiation effects* [Mesh] OR Telomere/radiation effects*[Mesh] OR Chromatin/radiation effects*[Mesh])";

Search used for scoring was performed on 2/04/2018. This fourth citation-based set was divided into quartiles scored as follows: 3 to highest quartile, 2 to 2nd quartile, 1 to 3rd quartile, 0 to 4th quartile. The sets were merged and scores for each gene were constructed by adding the expert-based and citation-based scores. Genes with a score of 2 or higher were retained in the set.

# 5 The effect of excluding gene expression, mutation or copy number variation

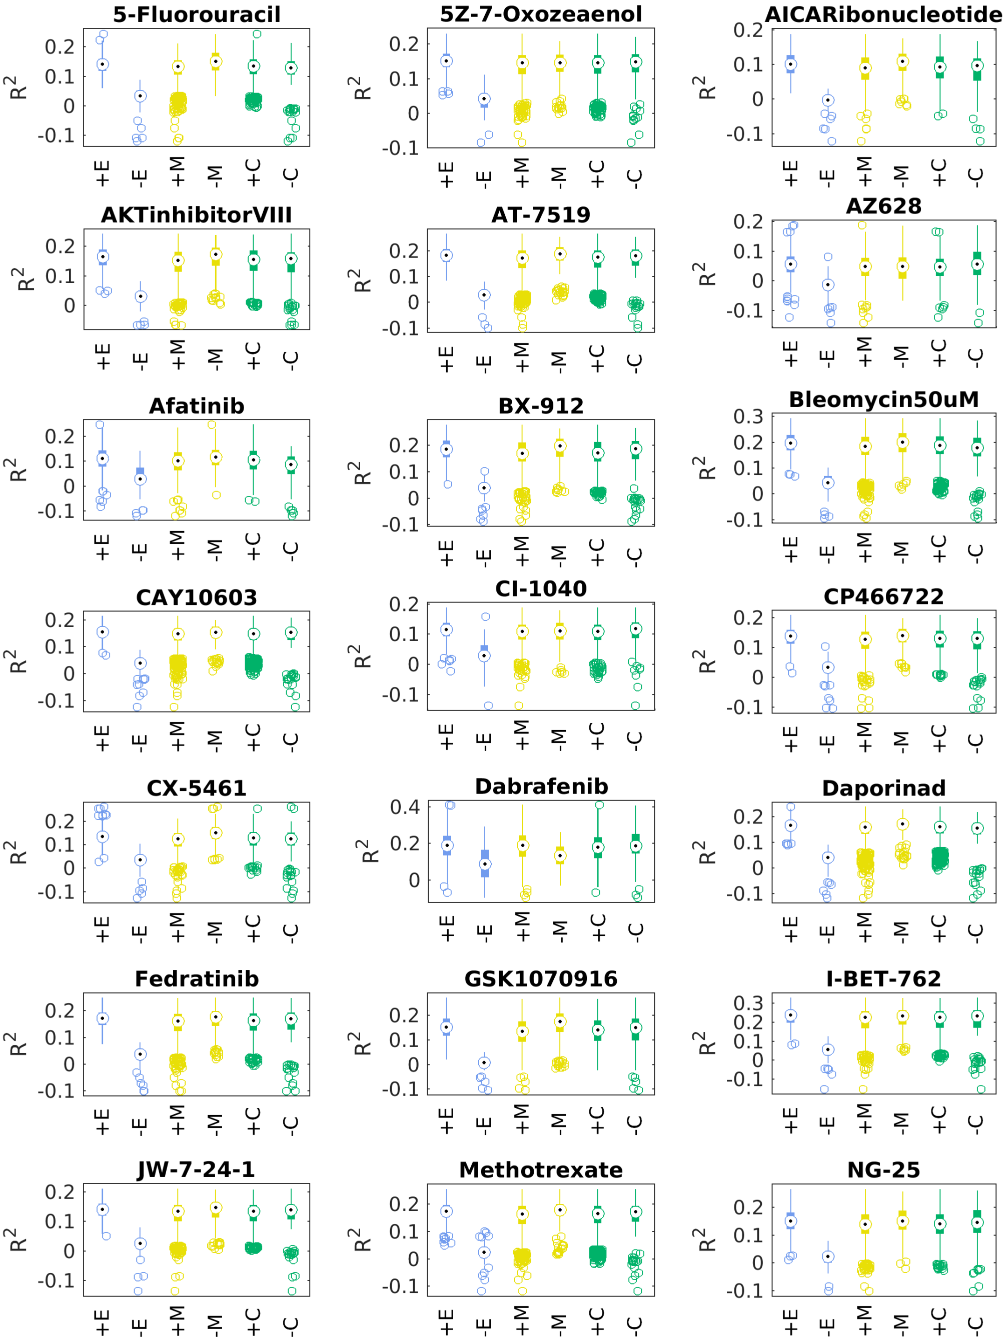


Figure 1: Distribution of $R^2$ obtained by all models and combos that do versus do not include gene expression (+E, -E, respectively), that do versus do not include mutation (+M and -M, respectively) and that do versus do not include copy number variation data (+C and -C, respectively). The figures show that for many drugs the distribution of $R^2$ for +E is higher than for -E. For mutation and copy number variation on the other hand there is hardly any difference between $R^2$ obtained with and without data of that feature type.

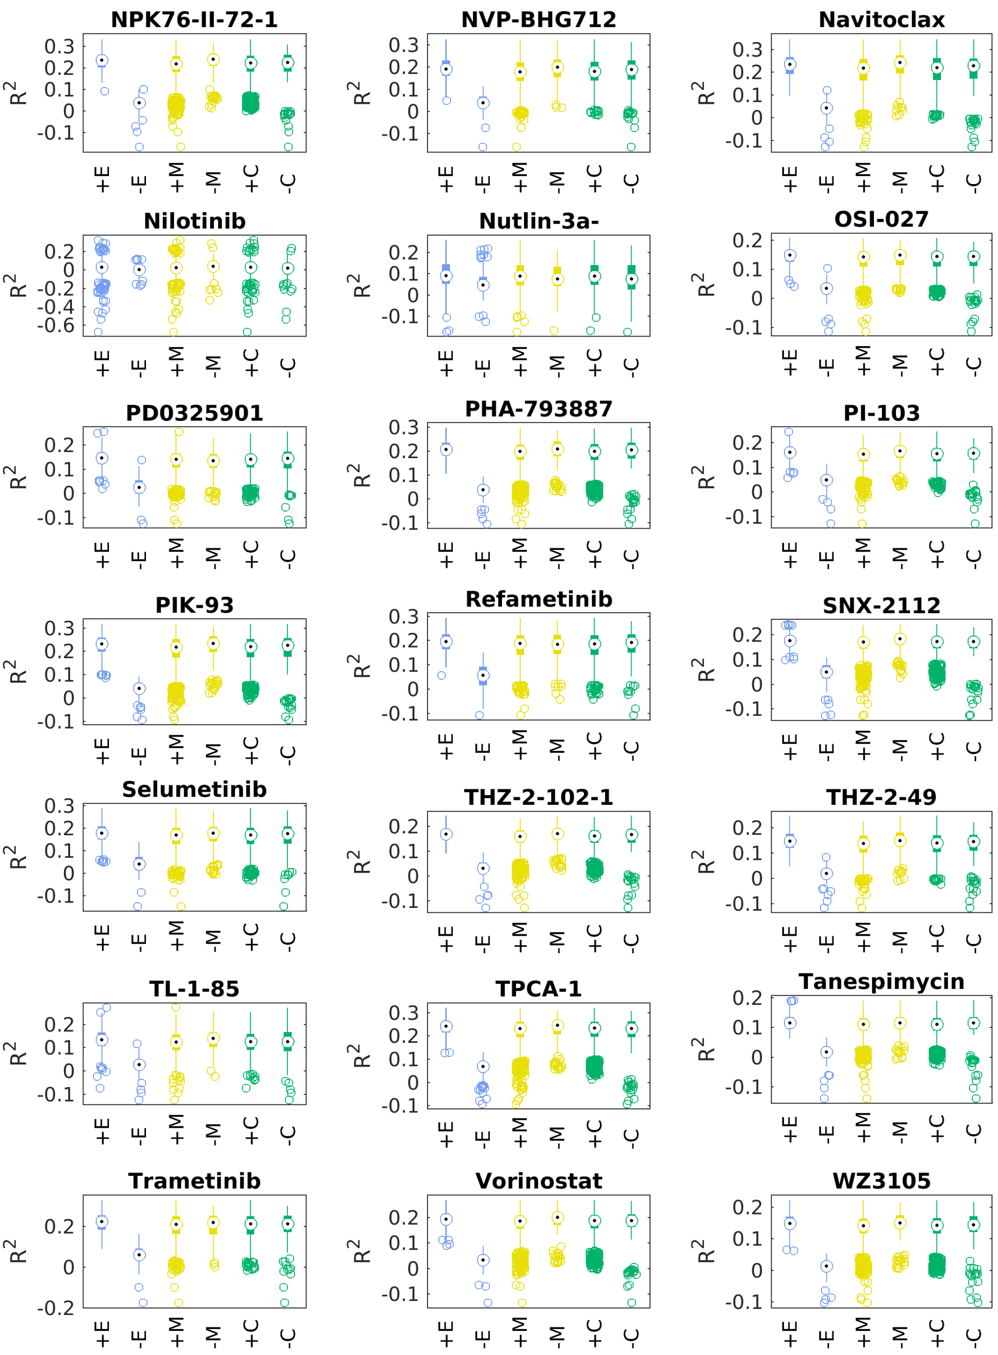


(Figure 1 continued.)

# 6 Feature importances

| | | | | | | | |
|---|---|---|---|---|---|---|---|
| 5-Fluorouracil | enet | eEGFR | eCREB1 | eMAP2K7 | ePLK3 | eTNF | eBAD |
| | rf | eGNA11 | eMET | eEGFR | eIKZF1 | eBTK | eRPL5 |
| 5Z-7-Oxozeaenol | enet | eSH2B3 | mBRAF | eFOXA1 | eSMO | eTGFBR2 | eZFHX3 |
| | rf | mBRAF | ePRKAR1A | eCDK2 | eSH2B3 | eFOXA1 | eCTNNB1 |
| AICARibonucleotide | enet | eMAX | eMYC | eCTNNB1 | cSFTPD | eWNT7A | eMKNK1 |
| | rf | eMYC | eIKZF1 | ePTEN | eCAT | eBLM | eMAX |
| AKTinhibitorVIII | enet | eEGFR | eACVR2A | eATP1A1 | eMET | eASXL1 | eNOTCH1 |
| | rf | eIKZF1 | ePRKCB | eMET | eGNA11 | eMAP4K1 | eDNMT3A |
| AT-7519 | enet | eTP53 | eIL6ST | eNOTCH1 | eKRAS | eCREB1 | eGABPB2 |
| | rf | eLSP1 | eGABPB1 | eIKZF1 | ePLK2 | eCCND1 | eBLM |
| AZ628 | enet | mBRAF | eBAD | ePARP2 | eBAX | eATM | mTGFB1 |
| | rf | eCTNNB1 | eWT1 | eTPP1 | ePYGL | eTAL1 | eZEB2 |
| Afatinib | enet | cERBB2 | eEGFR | eFGFR2 | cEGFR | eFGF2 | cCTNNB1 |
| | rf | eEGFR | eERBB2 | eSFN | ePGAP3 | cERBB2 | eCDH1 |
| BX-912 | enet | eCREB1 | eCDH1 | eIL6ST | eNEDD4L | eWRN | ePRKCB |
| | rf | eCREB1 | eMAP4K1 | ePRKCB | eEGFR | eIKZF1 | ePTEN |
| Bleomycin50uM | enet | eE2F1 | eTNFRSF10E | eBCL2L1 | ePRDX4 | eSMO | eGJA1 |
| | rf | eSERPINE1 | eE2F1 | eGJA1 | eSMO | eTNFRSF10E | eDRAM1 |
| CAY10603 | enet | eEGFR | eZFHX3 | ePTEN | eSMARCA4 | eCREB1 | eMAP2K7 |
| | rf | eMET | eEGFR | eERBB2 | eATP1B1 | eE2F2 | eBCL2 |
| CI-1040 | enet | mBRAF | ePRKCD | mNRAS | eZHX2 | ePARP2 | eGABPB1 |
| | rf | mBRAF | eMAD1L1 | eTPP1 | ePYGL | eCTNNB1 | eMLKL |
| CP466722 | enet | eIKBKB | eCREB1 | eTBX3 | eARID2 | eACVR2A | eRUNX1 |
| | rf | ePRKCB | eIKZF1 | ePTEN | eGNA11 | eBTK | eACVR2A |
| CX-5461 | enet | eTP53 | eNOTCH2 | ePLK3 | eBAD | eG6PD | eBAP1 |
| | rf | eMET | ePBRM1 | eRUNX1 | eDNMT3A | eBTK | eBAD |
| Dabrafenib | enet | mBRAF | eATM | eBCL2A1 | eATG5 | eMCL1 | eBAX |
| | rf | mBRAF | eBCL2A1 | eTPP1 | eATG5 | eSNAI2 | eCCND2 |
| Daporinad | enet | eOGT | eHNRNPA2B | eNCBP2 | cFGFR2 | eTRAF4 | eTSTA3 |
| | rf | eTHBS1 | ePLK2 | eTET1 | eEGFR | eBCL2L1 | eSFN |
| Fedratinib | enet | eCREB1 | eMYC | ePRKCB | ePLK2 | eIRF1 | eSFN |
| | rf | eMAP4K1 | eCREB1 | eMEF2C | eMEF2D | eJUN | eRAC1 |
| GSK1070916 | enet | eCREB1 | eIL6ST | eINSR | ePRKCB | eBID | ePRKCD |
| | rf | eFLT3 | eRUNX1 | eMET | eCXCR4 | eGNA11 | eARID2 |
| I-BET-762 | enet | eCREB1 | eMAP4K1 | eJUN | eMAP3K1 | eMEF2D | eMYC |
| | rf | eIKZF1 | eBTK | eGNA11 | ePTEN | eCD79B | eMET |
| JW-7-24-1 | enet | eCREB1 | eMYC | ePRKCB | eMDC1 | eSLC39A8 | eMAP4K5 |
| | rf | eIKZF1 | eCREB1 | ePRKCB | eMAP4K1 | eBTK | eMEF2C |
| Methotrexate | enet | eGNA11 | eSPEN | eERBB2 | eIL6ST | eSOCS1 | ePBRM1 |
| | rf | eIKZF1 | eCCND1 | eBRCA1 | eMET | eEGFR | eMYC |
| NG-25 | enet | eMYC | eGABPB1 | eJUN | eSFN | ePRKCB | eHRAS |
| | rf | eBTK | eIKZF1 | eMAP4K1 | eRAC1 | eMEF2C | eABL1 |
| NPK76-II-72-1 | enet | ePRKCB | eCREB1 | eWRN | eMYC | eSLC39A14 | eGABPB1 |
| | rf | ePRKCB | ePLK2 | eBLM | eGABPB1 | eIKZF1 | eCREB1 |

Figure 2: Top 6 feature importances for each drug and radiation as computed by elastic net and random forest. Gene name prefixes: e=expression, m=mutation, c=copy number. enet = elastic net, rf = random forest.

| | | | | | | | |
|---|---|---|---|---|---|---|---|
| NVP-BHG712 | enet | eCCND3 | eDCLRE1C | eATM | eBAD | eSFN | eBCL2L11 |
| | rf | eBTK | eIKZF1 | ePTEN | eABL1 | eCCND3 | ePRKCB |
| Navitoclax | enet | ePMAIP1 | eBCL2 | eGOT1 | eIDH2 | eCTNNB1 | eBAX |
| | rf | eBCL2 | eCCND1 | eBLM | eE2F2 | eE2F1 | eMCL1 |
| Nilotinib | enet | eWT1 | ePTCH1 | eSMO | eEML4 | eGNAS | eSOCS1 |
| | rf | eMKNK1 | eIKBKB | eMYC | eMAPK1 | eMAPK14 | eMAP3K7 |
| Nutlin-3a- | enet | eBAX | eMDM2 | eDDB2 | eCDKN2A | mTP53 | eXPC |
| | rf | mTP53 | eBAX | eMDM2 | eCDKN2A | ePYGL | eTNFSF10 |
| OSI-027 | enet | eEGFR | eE2F5 | eMYC | eTNFSF10 | eATM | eSH2B2 |
| | rf | eIKZF1 | eMET | eEGFR | eBTK | eCD79B | ePRKCB |
| PD0325901 | enet | eWNT5A | eZHX2 | eKRAS | eGABPB1 | eGJB1 | eSLC36A1 |
| | rf | ePYGL | eTPP1 | eBCL2A1 | eMAD1L1 | eCCND1 | eCTNNB1 |
| PHA-793887 | enet | eTBX3 | eKRAS | eEGFR | eUBR5 | eATM | eTP53 |
| | rf | eIKZF1 | eGNA11 | eACVR1 | eMET | eBTK | eCD79B |
| PI-103 | enet | eMYC | eSH2B2 | eATM | eBCL2L1 | eERBB2 | eMET |
| | rf | eIKZF1 | eMET | eCD79B | eBTK | eSH2B2 | eEGFR |
| PIK-93 | enet | eMYC | eATM | eEGFR | eMET | eBCL2 | ePRKCB |
| | rf | eBCL2 | eMET | eRB1 | ePRKCB | eEGFR | eE2F2 |
| Refametinib | enet | mBRAF | mKRAS | mNRAS | eTPP1 | eIGF1R | ePYGL |
| | rf | eCTNNB1 | eCDK2 | eTGFBR2 | eCCND1 | eTPP1 | mBRAF |
| SNX-2112 | enet | eGABPB1 | eTGFB1 | eBMPR1A | eATM | eBID | eMYC |
| | rf | ePRKCB | eMAP4K1 | eGABPB1 | eLSP1 | eMYC | eATM |
| Selumetinib | enet | ePARP2 | mBRAF | eGABPB1 | mKRAS | eIL6R | eZEB1 |
| | rf | eCTNNB1 | eTPP1 | eBCL2A1 | eE2F2 | ePYGL | eCCND1 |
| THZ-2-102-1 | enet | eEGFR | eMYC | eATM | eTP53 | eBCL2L1 | eRELA |
| | rf | eATP1B1 | eEGFR | eRPS11 | eKRT7 | ePRKCB | eJCHAIN |
| THZ-2-49 | enet | eZHX2 | eSFN | eMYC | eAR | eCDKN2B | eSLC25A39 |
| | rf | eIKZF1 | ePRKCB | eGNA11 | eBTK | eBCL2L11 | eAR |
| TL-1-85 | enet | eMYC | eJUN | eSFN | ePRKCB | eJAK2 | eNFKBIA |
| | rf | eMAPK1 | eJUN | eMAP3K7 | eABL1 | eMAP4K1 | eMAPK14 |
| TPCA-1 | enet | eGNA11 | eVHL | eTBX3 | eMYC | eATM | eGNAS |
| | rf | eMAP4K1 | eIKZF1 | eGNA11 | eBTK | eRAC1 | eMET |
| Tanespimycin | enet | eTNFRSF1A | eG6PD | eTNFRSF10E | eKLF4 | ePIK3CA | ePRKCB |
| | rf | eTNFRSF1A | ePLK2 | eEGFR | eG6PD | eKLF4 | eBCL2 |
| Trametinib | enet | eTGFBR2 | eBAD | eFADD | mBRAF | eGABPB1 | eWNT5A |
| | rf | eCCND1 | eTGFBR2 | eCTNNB1 | eCDK2 | eGJB1 | eE2F2 |
| Vorinostat | enet | eTET1 | eIL6ST | ePLK2 | eFN1 | eBCL9L | eCCND1 |
| | rf | eEGFR | ePLK2 | eIKZF1 | eBCL9L | eJUN | eTHBS1 |
| WZ3105 | enet | eEGFR | ePRKCB | eDRAM1 | mCDK4 | eMYC | eGABPB2 |
| | rf | eEGFR | eE2F2 | ePLK2 | eMET | eIKZF1 | eCCND1 |
| radiation | enet | eCOPB2 | eSMARCA4 | ePTMA | eCANX | eCOL1A2 | eMTHFD2 |
| | rf | eSMARCA4 | ePTMA | ePAICS | eCOPB2 | eACLY | eMTHFD2 |

(Figure 2 continued.)

# 7 Univariate comparison

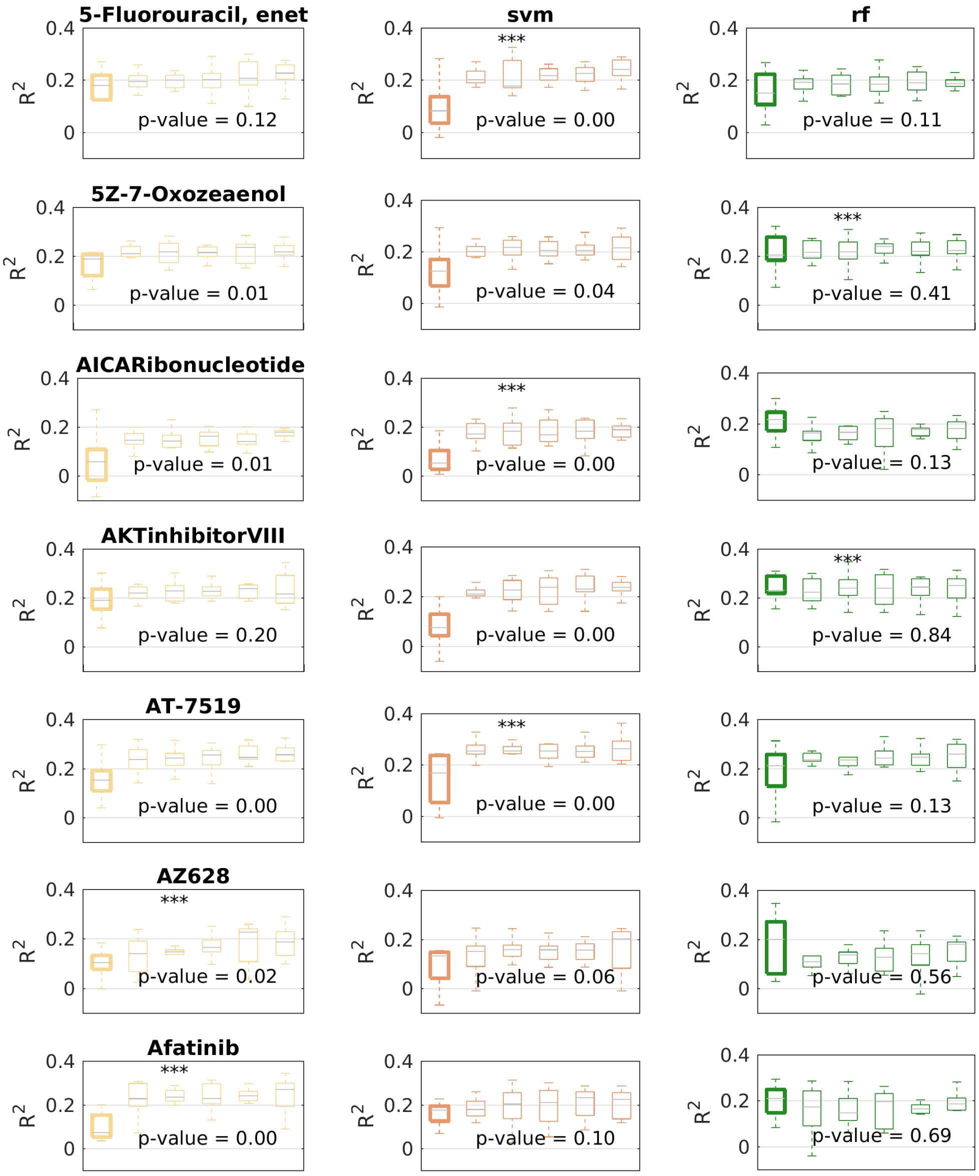


Figure 3: The distribution of $R^2$ over the 10 outer holdout loops for univariate feature selection (thick, left-most box plot) and the five top baseline (prior knowledge) results. The figures in the first, second and third column show the results for elastic net, support vector machine and random forest. The presented p-values correspond to the null hypothesis that $R^2$ obtained with the univariate gene selection approach is the same as the best $R^2$ values (rightmost) obtained with prior knowledge gene sets. In each row, the *** indicates which was the best algorithm for that drug, information which corresponds with that in main text Figure 1.

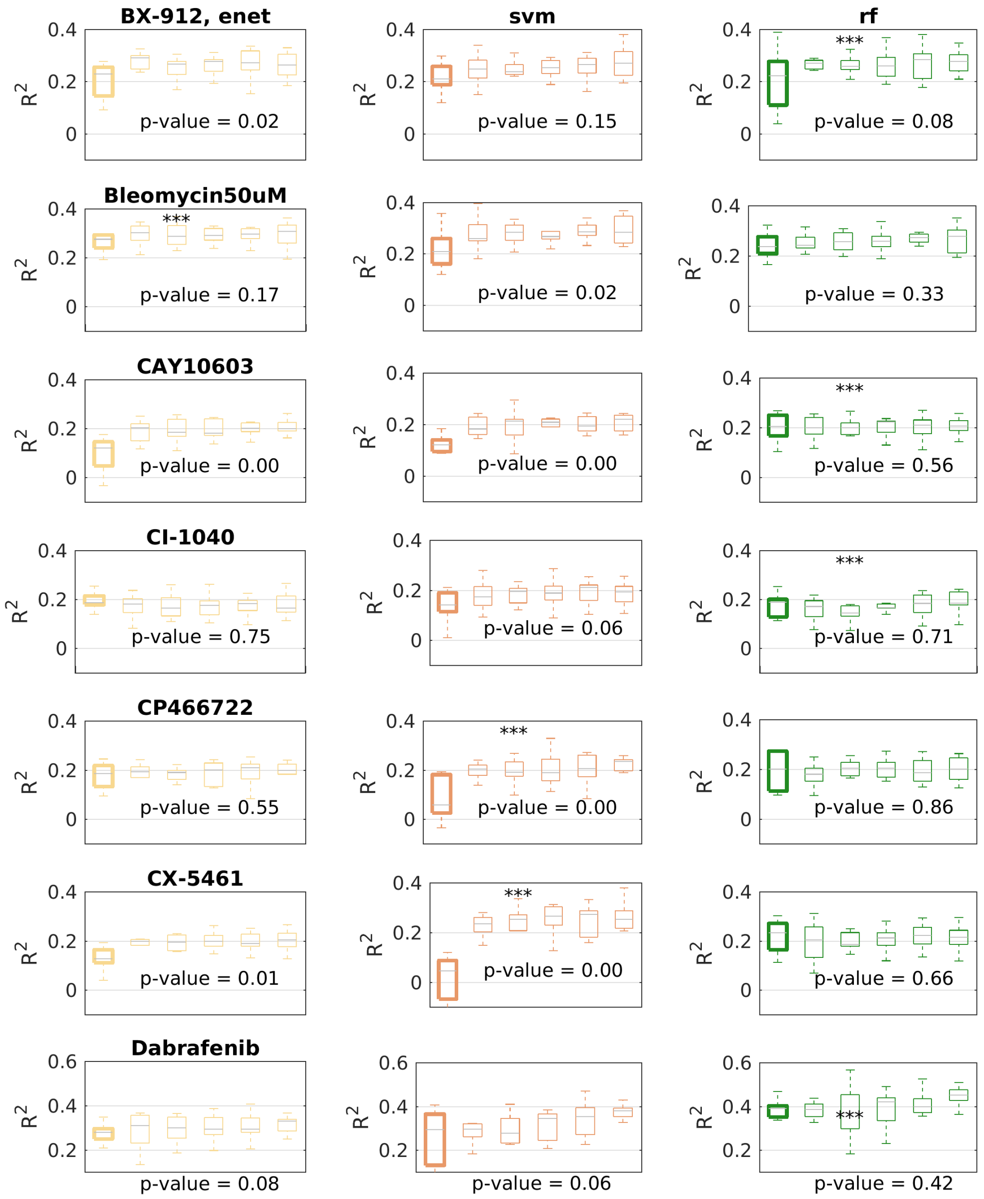


(Figure 3 continued.)

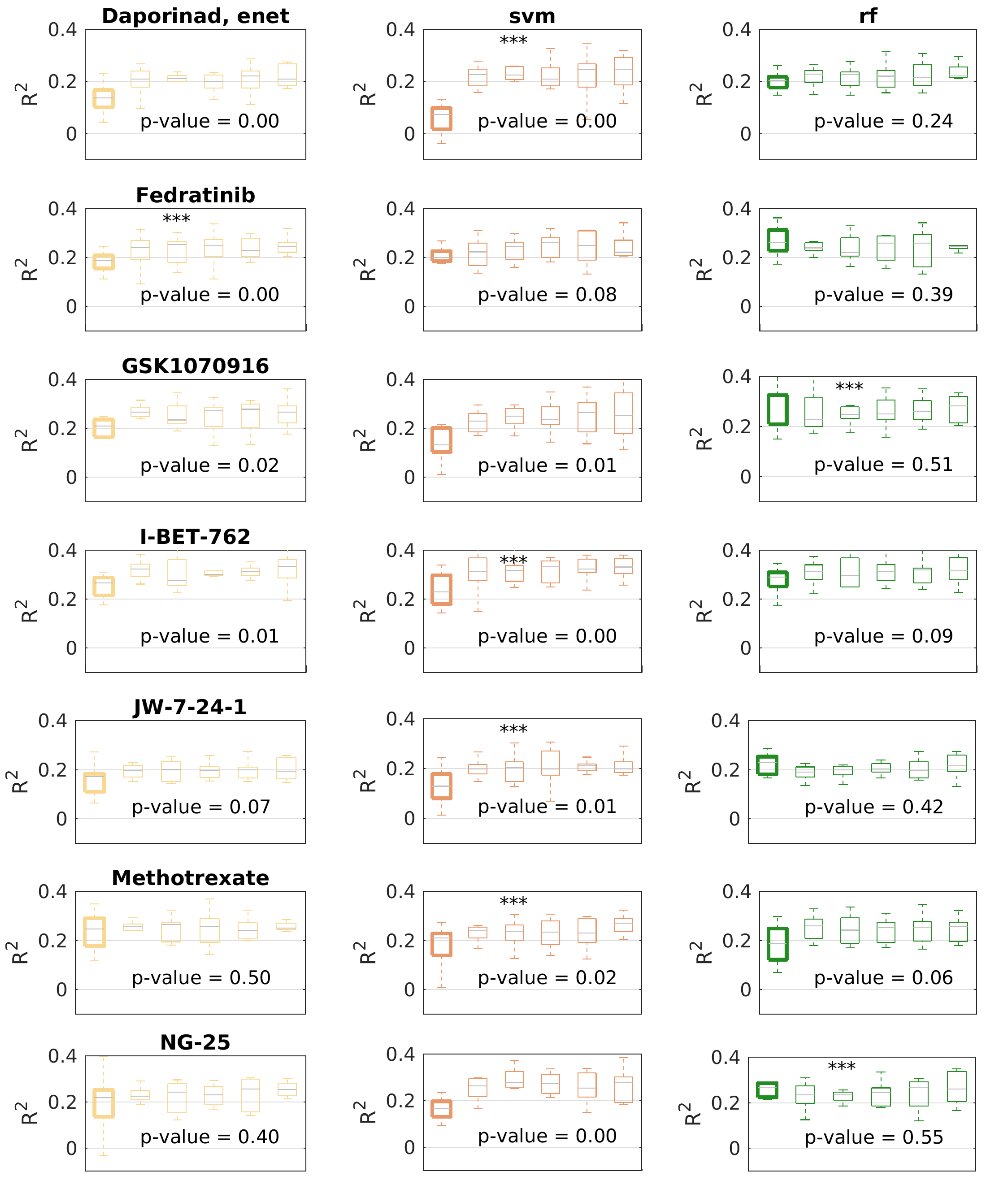


(Figure 3 continued.)

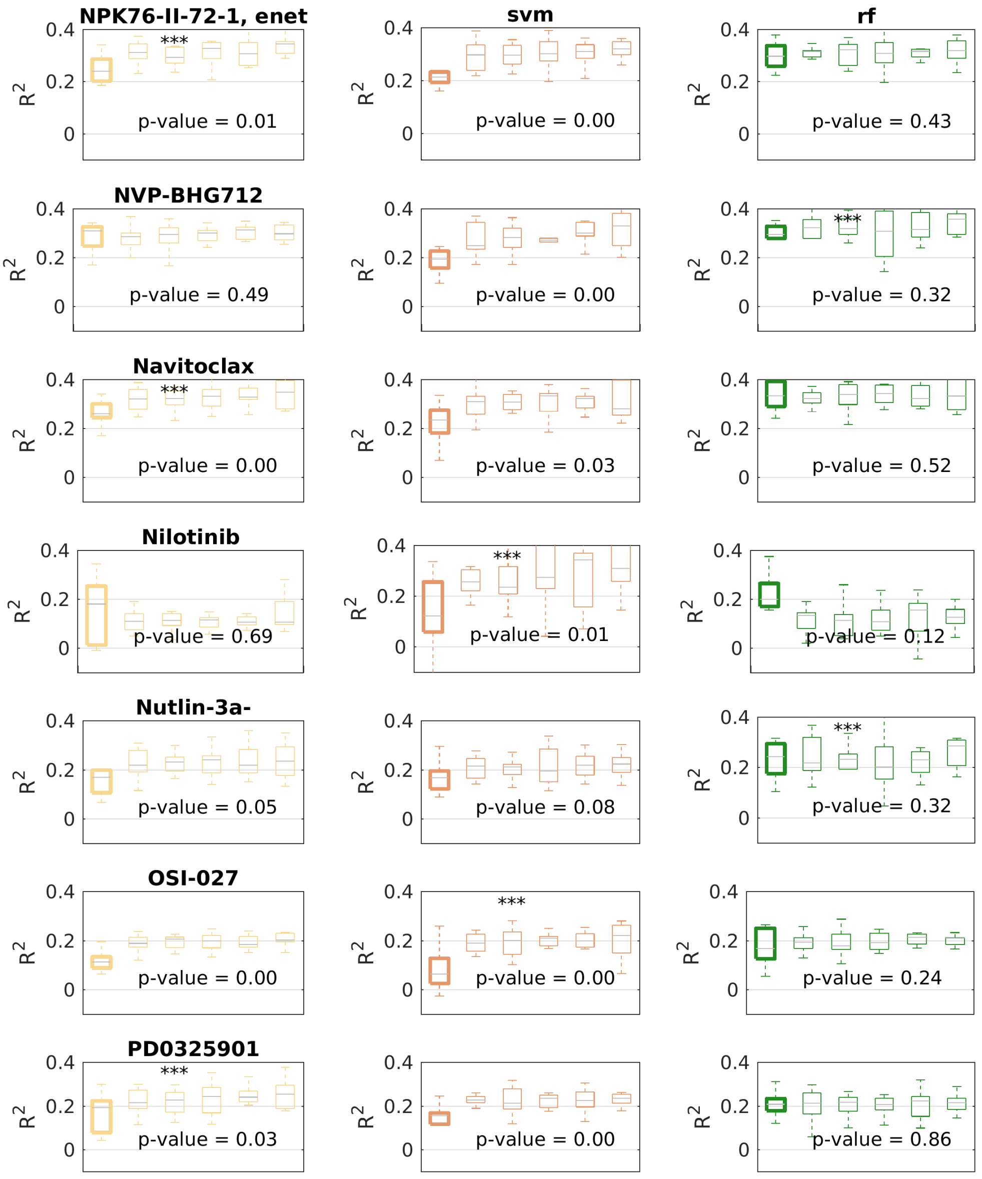


(Figure 3 continued.)

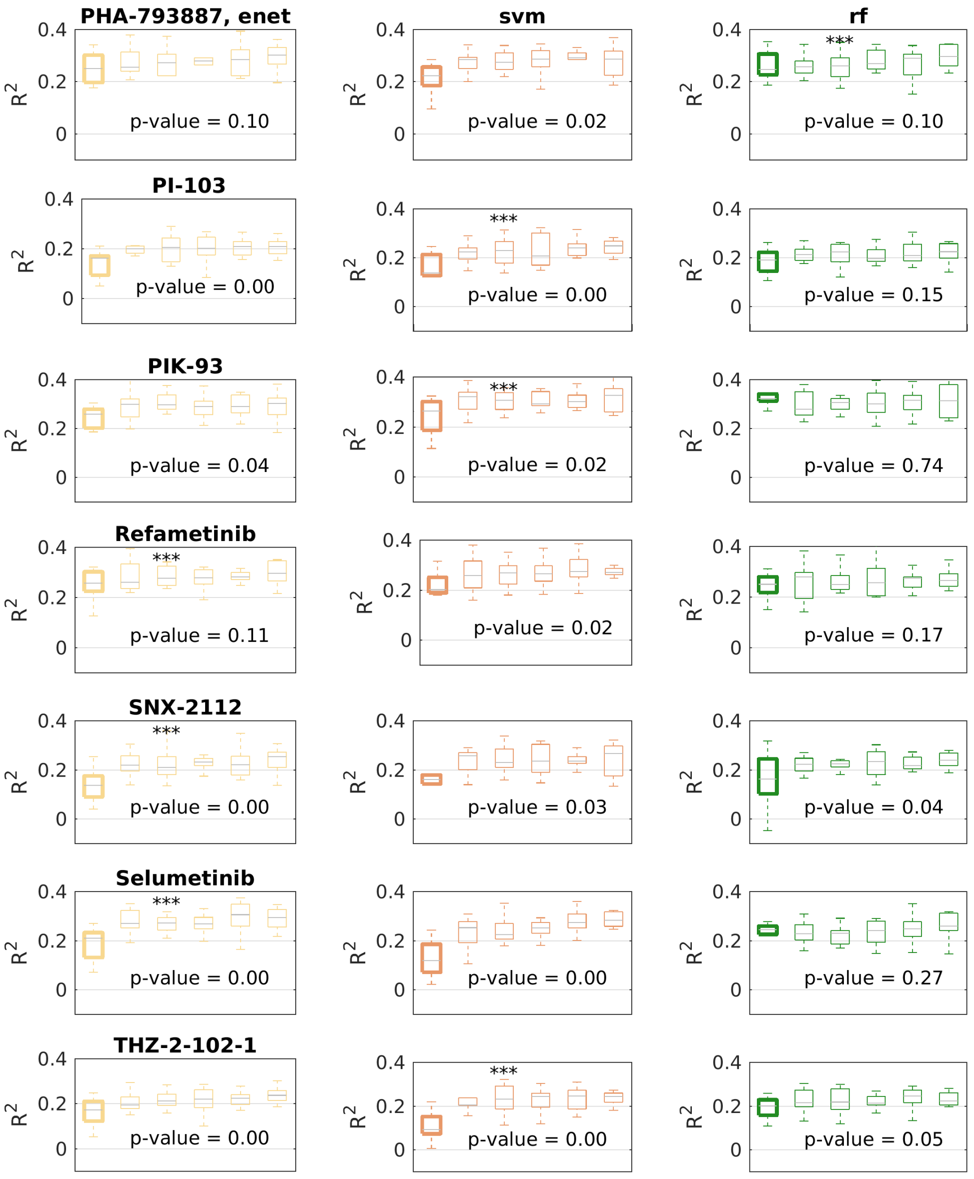


(Figure 3 continued.)

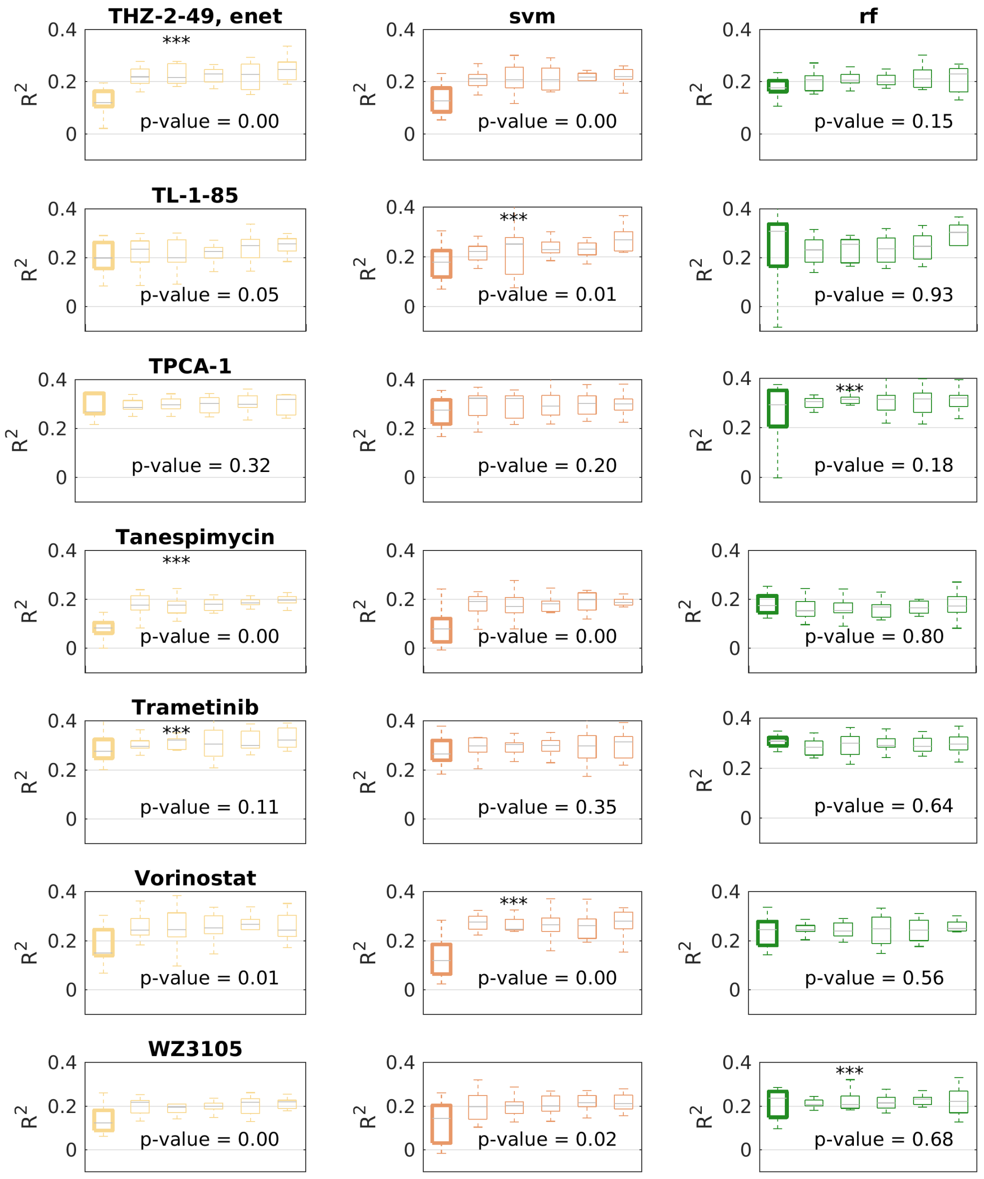


(Figure 3 continued.)

# 8 Type of encoding for mutation data does not influence prediction performance

Three drugs were chosen from the mid-range of predictability. For two of them (Selumetinib and Vorinostat), elastic net was the dominant algorithm, and for the third (TL-1-85) SVM was. In Figure 4, we plot the best outer loop baseline results for each drug alongside the best outer loop run, for the same algorithm, but with mutations coded as 0/1, and see that the encoding style does not influence the results. Similar results (not shown) for all algorithms (random forest, SVM, and elastic net) on these drugs.

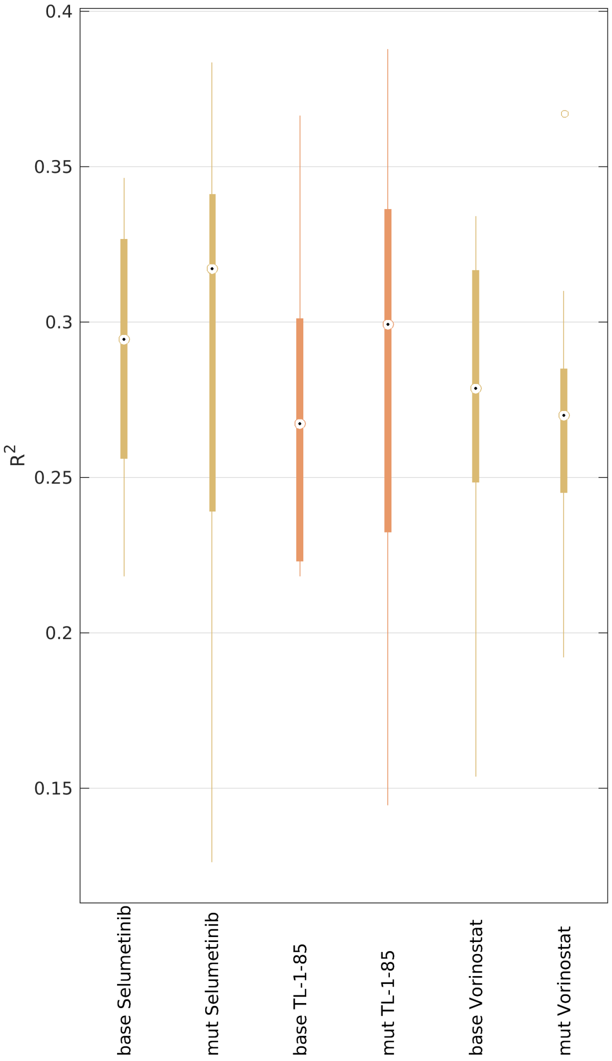


Figure 4: Prediction performance comparison for mutations 0/1 encoded versus baseline 7 category encoding. Drug prefix: base=baseline, mut = 0/1 mutation encoding. All p-values non-significant, indicating mutation encoding style does not affect the machine learning quality. Color scheme follows the standard: orange is SVM and yellow elastic net.

# 9 Including tissue type

In the Dr.S analysis, we compare our method against a simpler method which uses tissue type as the only cell line variable of interest, mimicking typical (non-genomic) clinical stratification. For three of the drugs CX-5461, NG-25, and PD0325901, chosen from the mid-range of predictability and chosen since they represent each of the three algorithm types (SVM, RF, and elastic net, respectively) as the best algorithm for that drug, we re-ran the baseline MAS analysis but included in every combo run an indicator variable for tissue type. For this we defined 25 types based on the two tissue type descriptors provided by the GDSC, see Table 9. The number of combos for these tissue type indicator variable runs is 343 (this is the baseline number of combos, 342, plus one combo for just tissue type encoding). For drug CX-5461 (SVM algorithm) and NG-25 (random forest) median $R^2$ is higher when tissue type is included, and for drug drug PD0325901 (elastic net), baseline result is higher, but none of these differences is significant, see Figure 5. Also, for each drug, the dominant algorithm when tissue type indicator variable is included is the same as the dominant algorithm in the baseline runs.

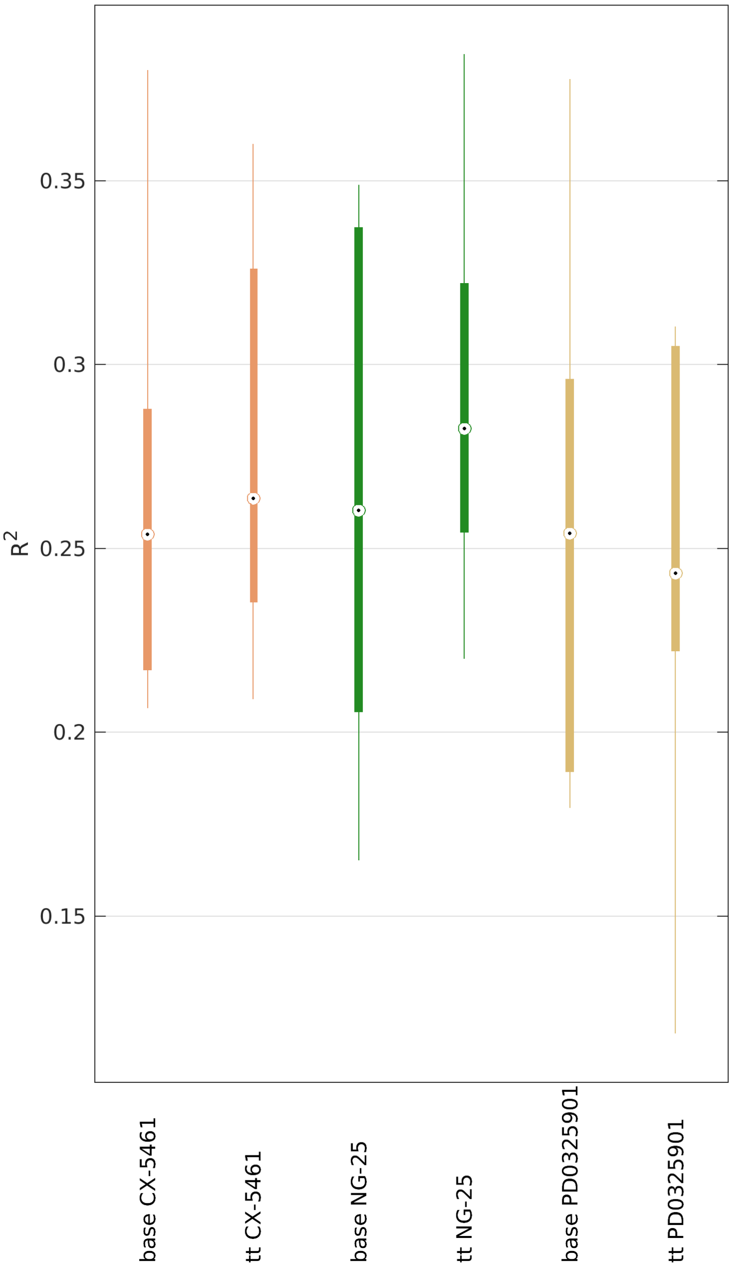


Figure 5: For three drugs, best baseline results compared with best results when including tissue type as a one-hot encoded indicator variable. base=baseline, tt=tissue type one hot encoding included. Color scheme follows the standard: orange is SVM, green Random Forest, and yellow Elastic Net.

Table 9: Definition of tissue types for cell line classification.

| Tissue type ID | GDSC tissue descriptor 1 | GDSC tissue descriptor 2 | Number of cell lines |
|---|---|---|---|
| 1 | aero_dig_tract | head and neck | 44 |
| 2 | aero_dig_tract | oesophagus | 35 |
| 3 | bone | bone_other | 3 |
| | bone | chondrosarcoma | 5 |
| | bone | ewings_sarcoma | 22 |
| | bone | osteosarcoma | 10 |
| 4 | breast | breast | |
| 5 | digestive_system | biliary_tract | 5 |
| | digestive_system | digestive_system_other | 1 |
| 6 | digestive_system | liver | 17 |
| 7 | digestive_system | stomach | 29 |
| 8 | kidney | adrenal gland | 1 |
| | kidney | kidney | 33 |
| 9 | large_intestine | large_intestine | 51 |
| 10 | lung | Lung_other | 1 |
| | lung | mesothelioma | 21 |
| 11 | lung_NSCLC | lung_NSCLC_adenocarcinoma | 67 |
| | lung_NSCLC | lung_NSCLC_carcinoid | 4 |
| | lung_NSCLC | lung_NSCLC_large cell | 14 |
| | lung_NSCLC | lung_NSCLC_not specified | 11 |
| | lung_NSCLC | lung_NSCLC_squamous_cell_carcinoma | 15 |
| 12 | lung_SCLC | lung_small_cell_carcinoma | 66 |
| 13 | lymphoma | B_cell_lymphoma | 35 |
| | lymphoma | Burkitt_lymphoma | 13 |
| | lymphoma | Hodgkin_lymphoma | 9 |
| | lymphoma | anaplastic_large_cell_lymphoma | 3 |
| 13 | lymphoma | lymphoid_neoplasm other | 10 |
| 14 | myeloma | haematopoietic_neoplasm other | 4 |
| | myeloma | lymphoid_neoplasm other | 1 |

| Tissue type ID | GDSC tissue descriptor 1 | GDSC tissue descriptor 2 | Number of cell lines |
|---|---|---|---|
| | myeloma | myeloma | 13 |
| 15 | nervous_system | glioma | 53 |
| | nervous_system | medulloblastoma | 4 |
| 16 | neuroblastoma | neuroblastoma | 32 |
| 17 | pancreas | pancreas | 32 |
| 18 | skin | melanoma | 55 |
| | skin | skin_other | 3 |
| 19 | soft_tissue | fibrosarcoma | 3 |
| | soft_tissue | rhabdomyosarcoma | 9 |
| | soft_tissue | soft_tissue_other | 9 |
| 20 | thyroid | thyroid | 16 |
| 21 | urogenital_system | Bladder | 19 |
| 22 | urogenital_system | cervix | 15 |
| | urogenital_system | endometrium | 11 |
| | urogenital_system | ovary | 43 |
| | urogenital_system | uterus | 2 |
| 23 | urogenital_system | prostate | 8 |
| | urogenital_system | testis | 3 |
| 24 | urogenital_system | urogenital_system_other | 4 |
| 25 | leukemia | B_cell_leukemia | 13 |
| | leukemia | T_cell_leukemia | 4 |
| | leukemia | acute_myeloid_leukaemia | 27 |
| | leukemia | chronic_myeloid_leukaemia | 10 |
| | leukemia | haematopoietic_neoplasm other | 2 |
| | leukemia | hairy_cell_leukaemia | 4 |
| | leukemia | leukemia | 4 |
| | leukemia | lymphoblastic_T_cell_leukaemia | 9 |
| | leukemia | lymphoblastic_leukemia | 12 |

# 10 Radiation results

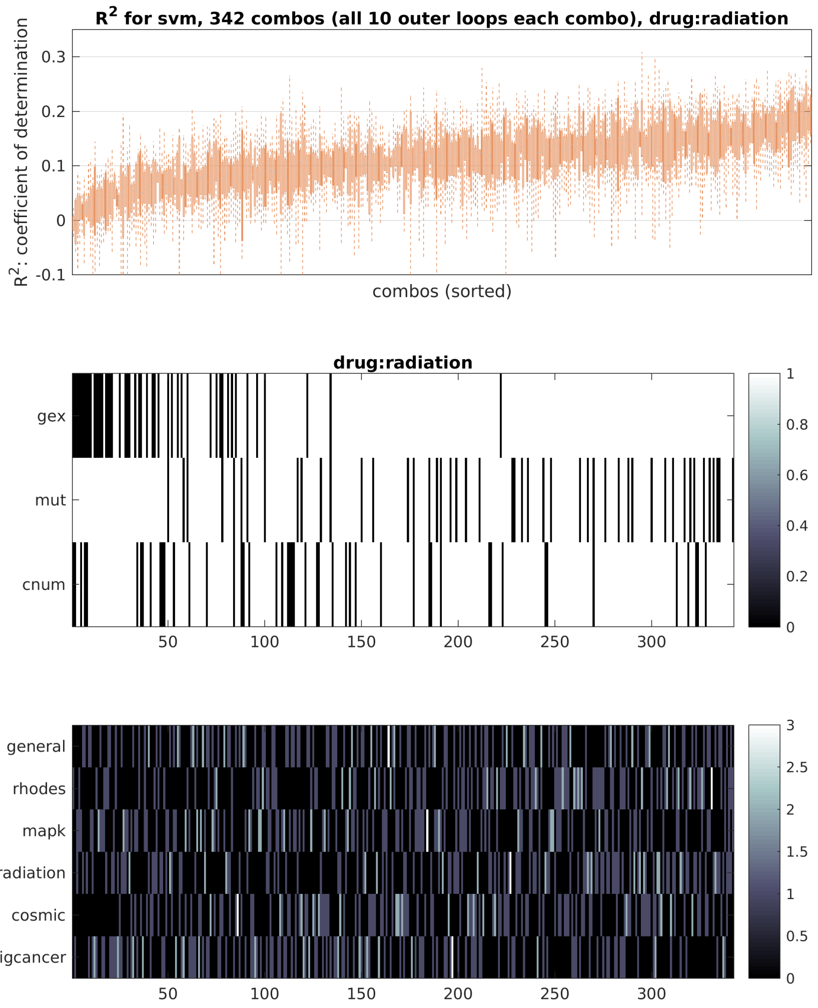


Figure 6: SVM results for the radiation run. Top panel: all combos sorted by mean $R^2$ from outer loop. Middle panel: in the same sorted combo order, a display of which feature types are used for each combo. Visually can observe that the worst combos (leftmost) are the ones where gene expression is not included (black). Bottom panel: in the same sorted order, for each combo we display how many times (up to three) the particular gene set was used.

# 11 Random gene sets and gene set size investigations

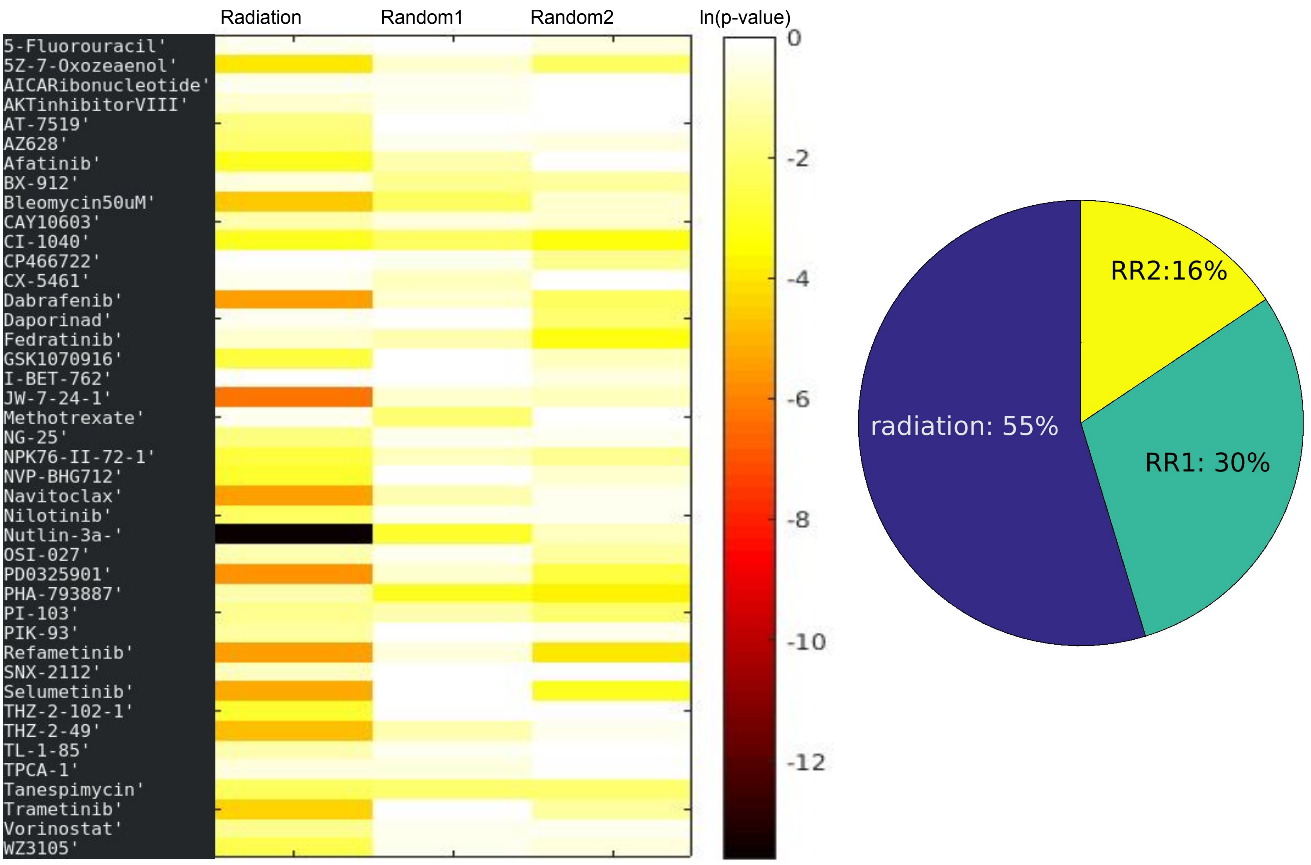


Figure 7: Results of running all 42 drugs with three gene sets: the radiation gene set and two random gene sets of the same length as the radiation set, 263 genes. For each drug we compare the $R^2$ values with and without each set (all combos included, not just top combos). The heatmap shows the natural log of the p-value for the rank sum test for the set of runs with a gene set and without. The pie graph shows the relative usage frequency of each set in the single top combo for each drug.

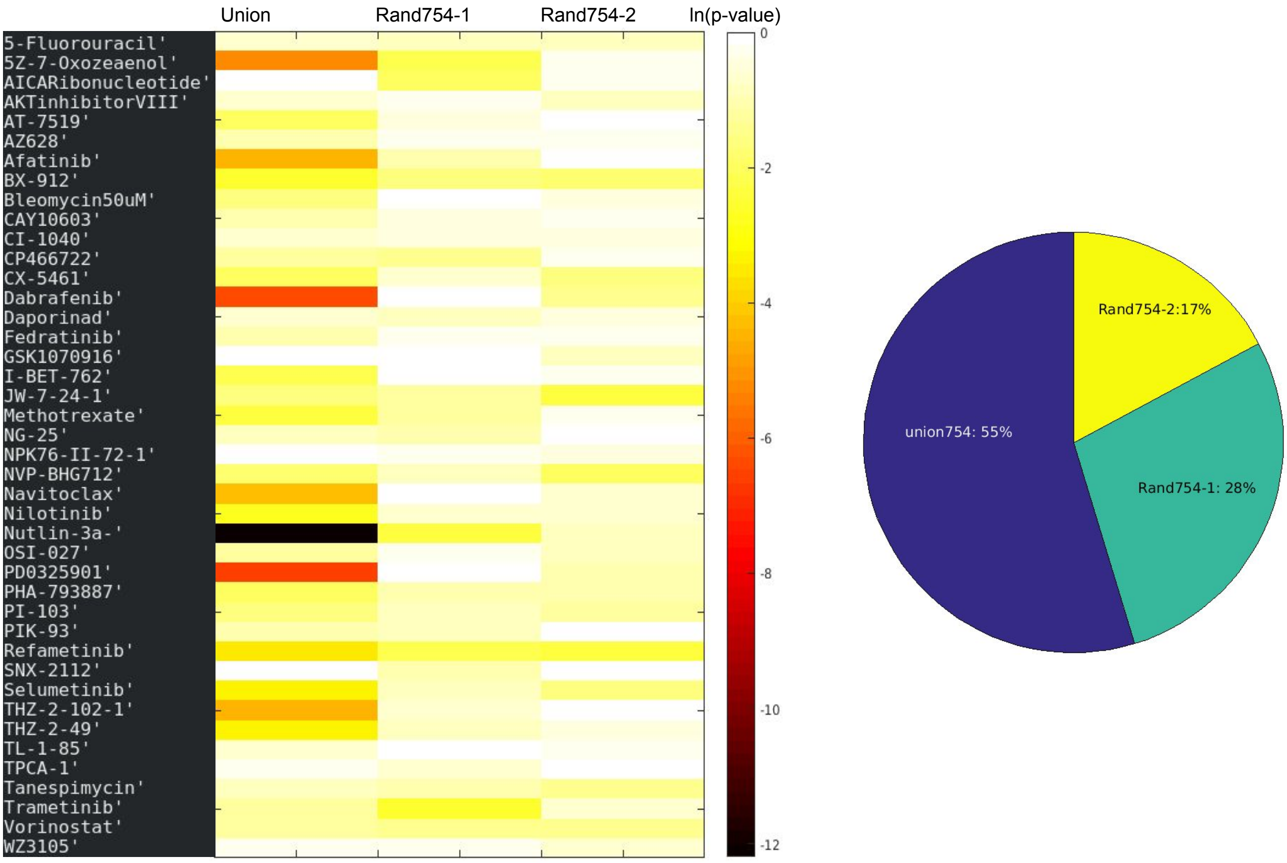


Figure 8: Results of running all 42 drugs with three gene sets: the union gene set and two random gene sets of the same length as the union set, 754 genes. For each drug we compare the $R^2$ values with and without each set (all combos included, not just top combos). The heatmap shows the natural log of the p-value for the rank sum test for the set of runs with a gene set and without. The pie graph shows the relative usage frequency of each set in the single top combo for each drug.

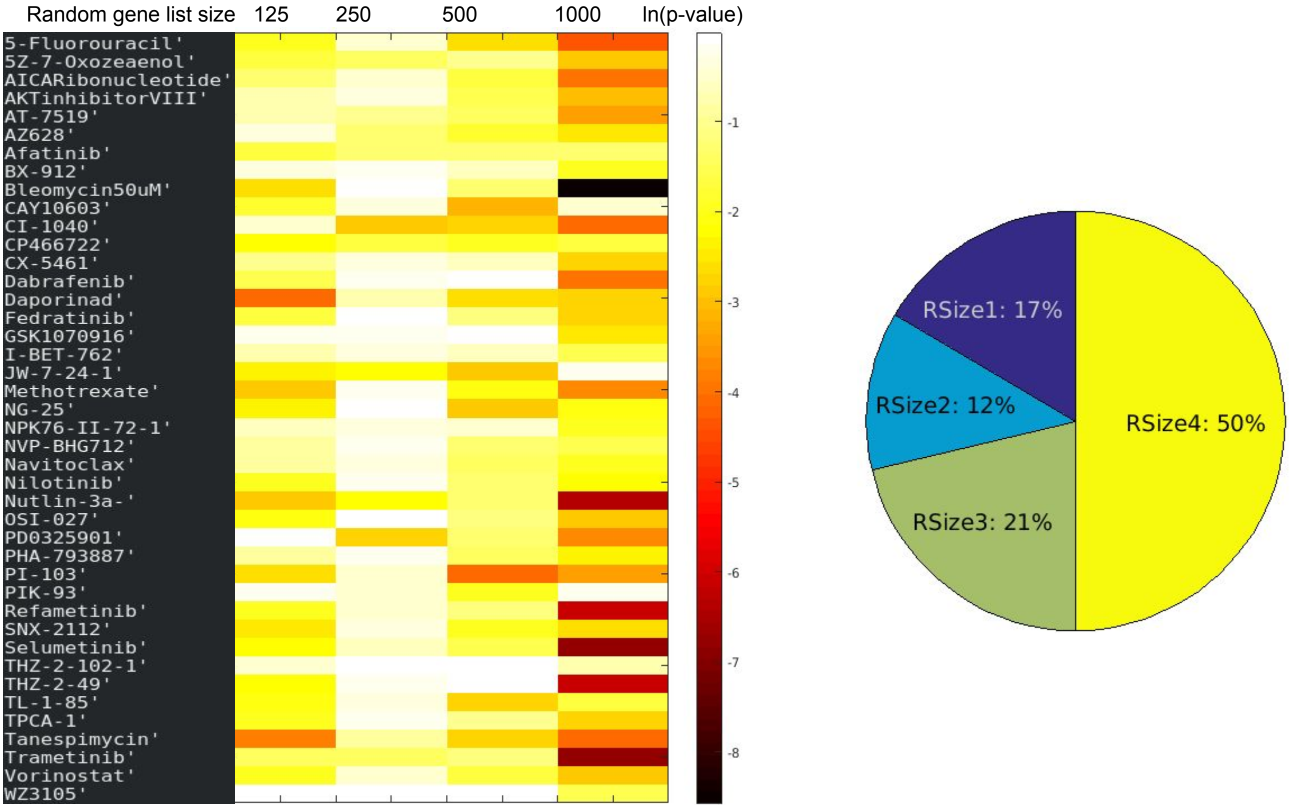


Figure 9: Results of running all 42 drugs with four gene sets of increasing size. For each drug we compare the $R^2$ values with and without each set (all combos included, not just top combos). The heatmap shows the natural log of the p-value for the rank sum test for the set of runs with a gene set and without. The pie graph shows the relative usage frequency of each set in the single top combo for each drug. RSize1 is the random 125 gene lists, RSize2 is the next largest, etc.

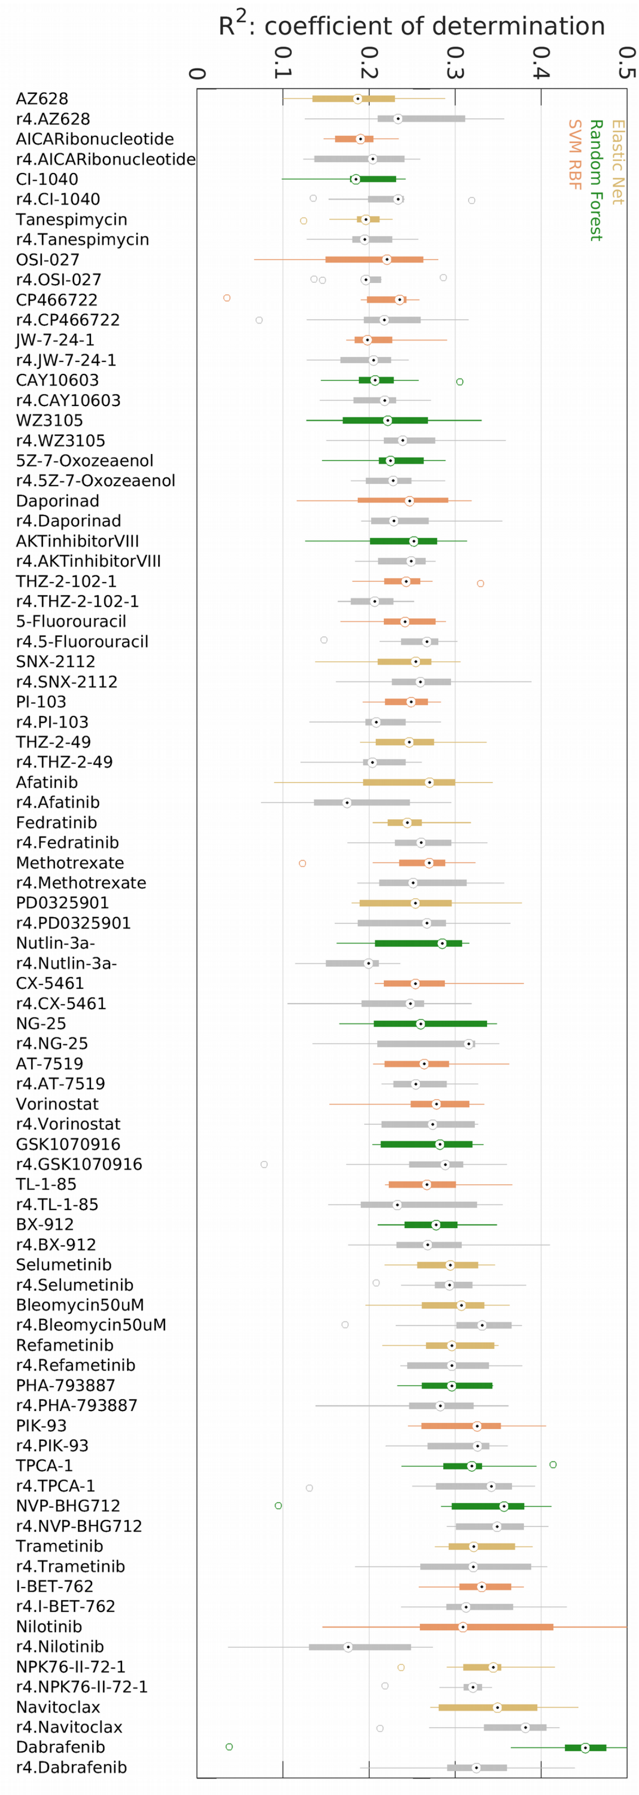


Figure 10: Baseline MAS results (colored) aside best of the [random 125, 250, 500, 1000] gene run combos (gray).

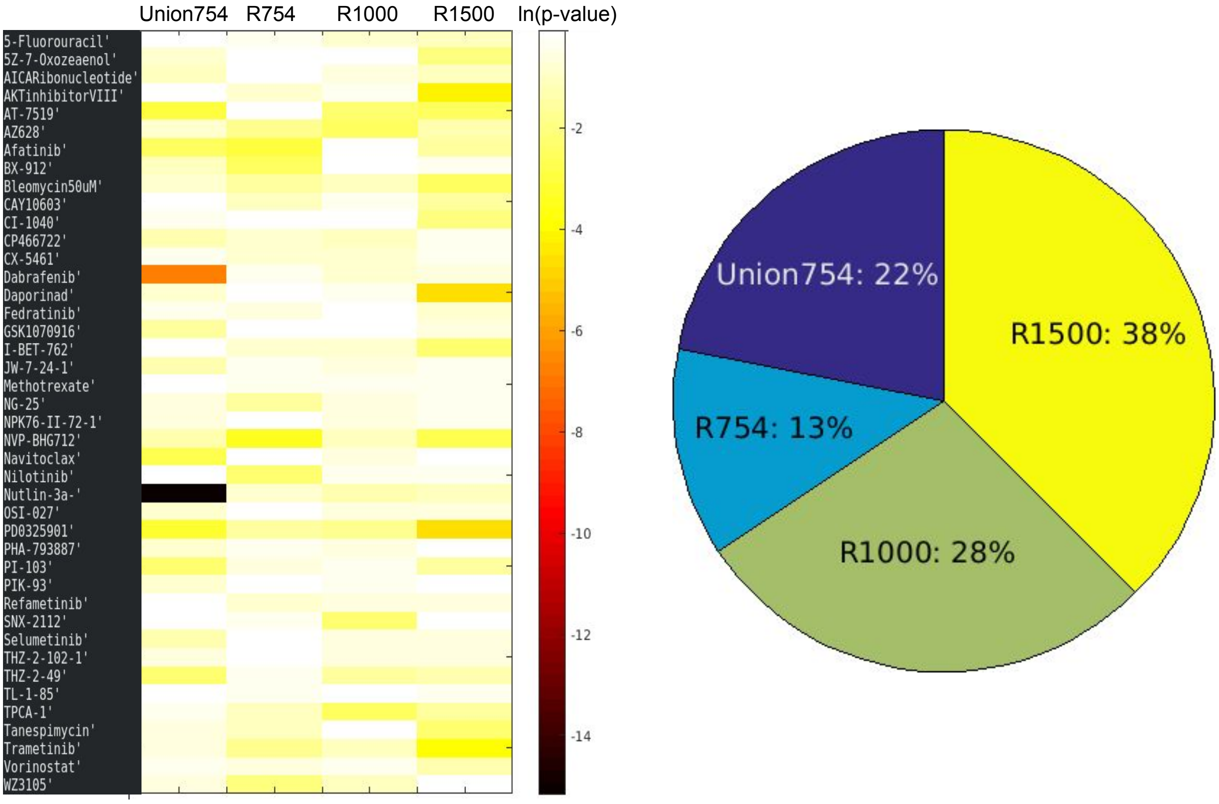


Figure 11: Results of running all 42 drugs with the following four gene set: union of curated sets, random set of size 754, random of size 1000, and random of size 1500. For each drug we compare the $R^2$ values with and without each set (all combos included, not just top combos). The heatmap shows the natural log of the p-value for the rank sum test for the set of runs with a gene set and without. The pie graph shows the relative usage frequency of each set in the single top combo for each drug.

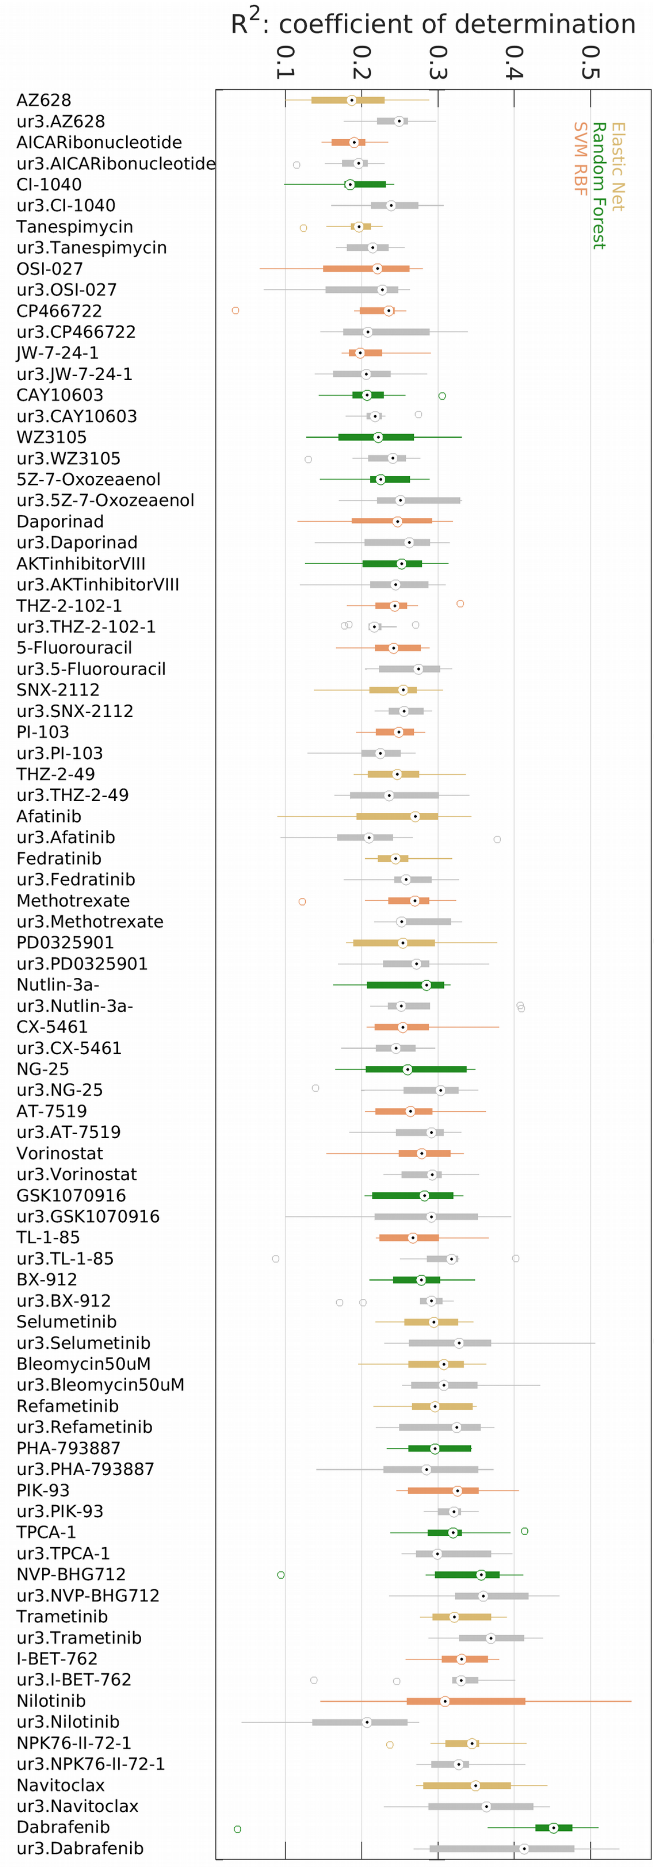


Figure 12: Baseline MAS results (colored) aside best of the [union 754, random 754, random 1000, random 1500] run combos (gray).

## 12 Performance of Dr.S compared to tissue type based recommendations

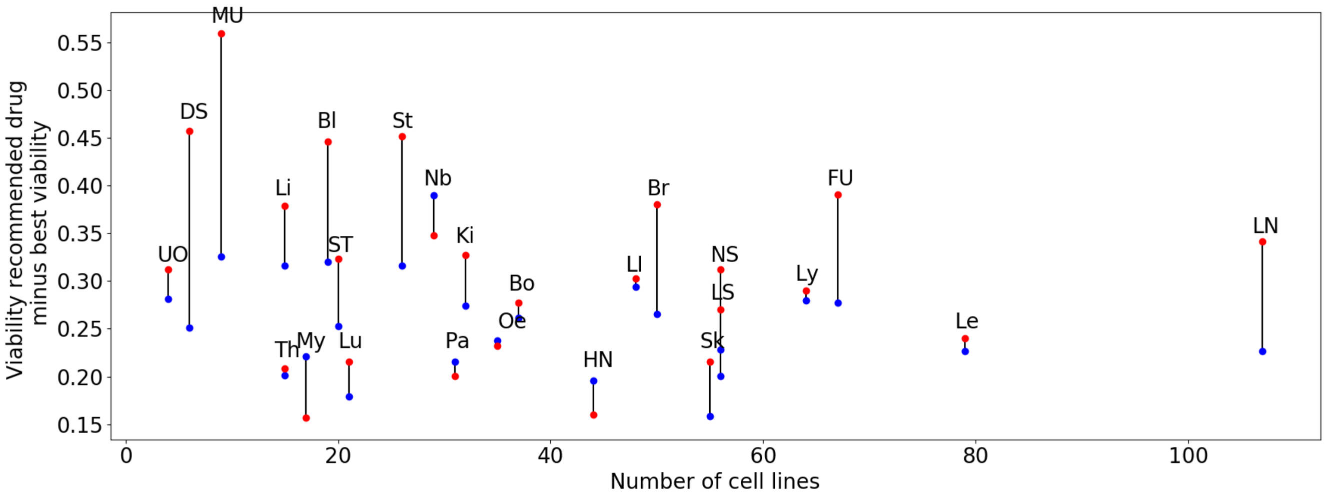


Figure 13: Viability recommended drug by Dr.S (blue) or the tissue type based prescription (red) minus the viability of the true best drug, averaged over all cell lines with the same tissue type. The blue and red dot that correspond to the same tissue type are connected. Acronyms for tissue types: Bo = Bone, Bl = Bladder, Br = Breast, DS = Digestive system, FU = Female urogenital system, HN = Head & Neck, Ki = Kidney, Le = Leukemia, Li = Liver, LI = Large intestine, Lu = Lung, LN = Lung NSCLC, LS = Lung SCLC, Ly = Lymphoma, MU = Male urogenital system, My = Myeloma, Nb = Neuroblastoma, NS = Nervous system, Oe = Oesophagus, Pa = Pancreas, Sk = Skin, St = Stomach, ST = Soft tissue, Th = Thyroid, UO = Urogenital system other.

# 13 Recommending drugs with viability at most $\varepsilon$ higher than the best drug

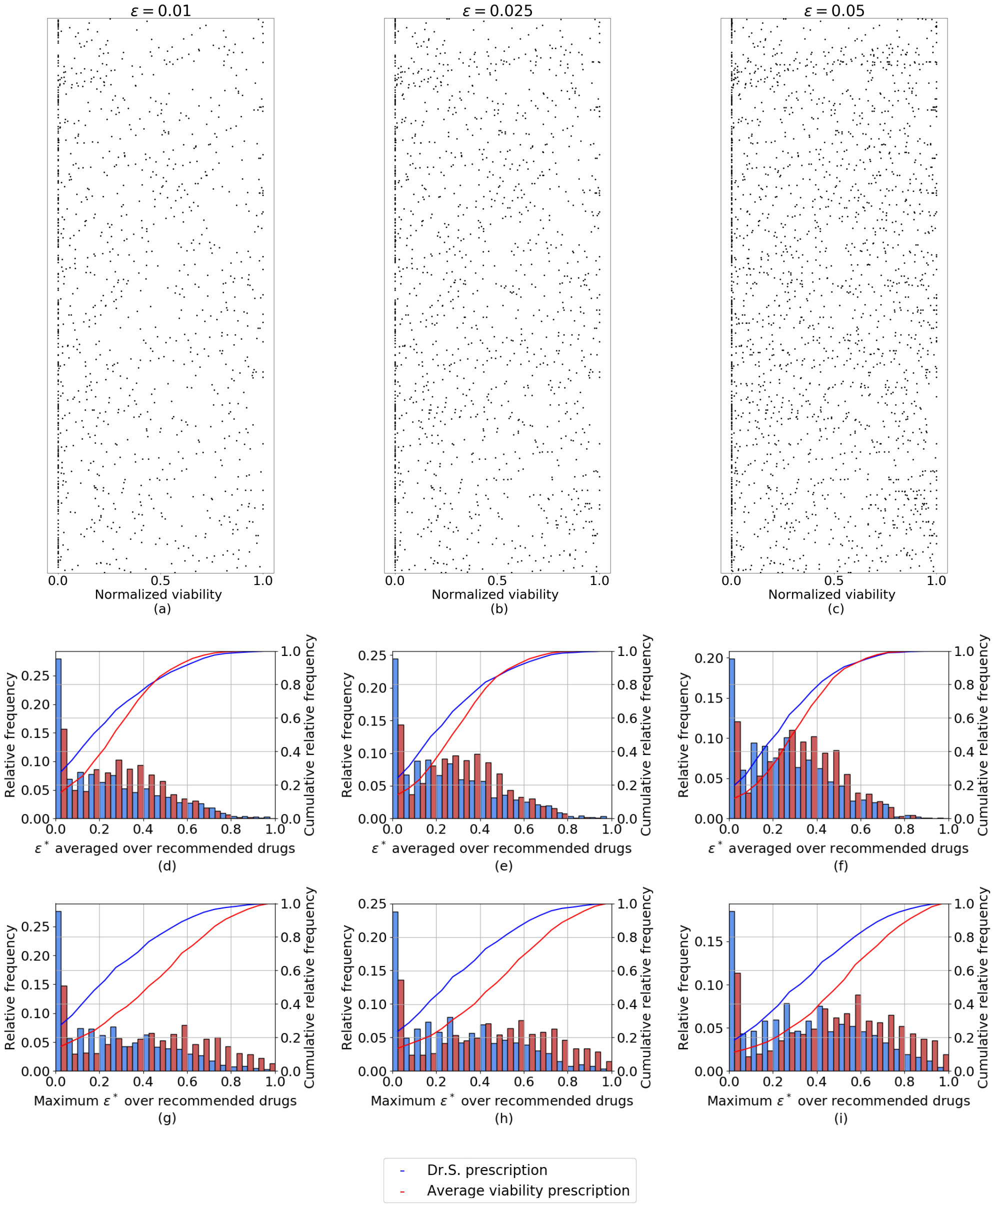


Figure 14: Results obtained with Dr.S and tissue type based prescription where all drugs with a predicted viability within $\varepsilon$ of the best predicted viability are in the prescription. Figures (a), (d) and (g) correspond to $\varepsilon = 0.01$, (b), (e) and (h) to $\varepsilon = 0.025$ and (c), (f) and (i) to $\varepsilon = 0.05$. In Figures (a)-(c) each row corresponds to a cell line, and the dots indicate the normalized viability of the recommended drugs where a normalized viability of 0 (1) corresponds to the viability of the best (worst) drug. Figures (d)-(f) show the (cumulative) distribution of $\varepsilon^*$ over the cell lines, averaged over the set of recommended drug for that cell line. Figures (g)-(i) show the (cumulative) distribution over the cell lines of the maximum $\varepsilon^*$ over the recommended drug for that cell line.

# 14 Literature review

Two major cell line datasets were constructed in 2012: the GDSC [Yang et al., 2013, Garnett et al., 2012] and the CCLE [Barretina et al., 2012]. The corresponding papers provided a preliminary analysis of these data, where the aim was to identify the genomic features that were associated with sensitivity. For this a multivariate analysis of variance (MANOVA) and an elastic net analysis were carried out on the respective datasets. Soon many research groups began to develop and test drug sensitivity prediction models for these datasets. In these studies the primary goal was to develop prediction methods that achieved a high predictive performance, while identification of sensitivity-inducing genomic characteristic became a secondary goal.

A wide variety of models has been employed for the prediction of drug sensitivity for cell lines. Initially several variants of linear regression, such as elastic net and ridge regression, were applied. Soon after the initial publications of the GDSC and CCLE non-linear methods were applied, of which random forest (RF) and support vector machine (SVM) are often-used examples. When choosing a machine learning method it is important to decide whether one aims to predict a continuous (e.g. IC50) or a discrete outcome (e.g. sensitive versus resistant).

A major complicating factor in drug sensitivity prediction is the curse of dimensionality: the number of genomic features (on the order of $10^4$-$10^5$) largely exceeds the number of cell lines (fewer than 1,000). Some studies resolve this issue by pre-selecting features based on prior knowledge, e.g. by including only information from oncogenes [Iorio et al., 2016, Chen and Sun, 2017, Suphavilai et al., 2018]. Others develop a method to select features using correlation with sensitivity, recursive feature elimination or subset evaluation techniques [Papillon-Cavanagh et al., 2013, Jeon et al., 2014, Gupta et al., 2016, Dong et al., 2015]. Others summarize the input data by considering principal components [Jang et al., 2014] or computing pathway activity scores [Yang et al., 2013, Wang et al., 2019].

Initially machine learning models were developed and trained to predict drug sensitivity of a particular drug for new cell lines from their genomic information. At the other end quantitative structure-activity relationship (QSAR) models predict the response of a biological entity to a new drug based on physico-chemical properties of a drug. Several studies have combined the two approaches into a "multi-task" drug sensitivity problem [Gönen and Margolin, 2014, Menden et al., 2013, Yang et al., 2018, Costello et al., 2014, Zhang et al., 2018, Cortés-Ciriano et al., 2015, Tan, 2016], where multi-task refers to the models being trained on predicting sensitivity for multiple drugs simultaneously. Several studies build a multi-task learning approach where each sample is a cell line-drug combination for which both genomic features and physico-chemical properties of drugs are included as independent variables [Zhang et al., 2018, Menden et al., 2013, Cortés-Ciriano et al., 2015]. Other studies use a recommendation system where the prediction is based on information

from the response matrix [Gönen and Margolin, 2014, Yang et al., 2018, Costello et al., 2014].

With the proliferation of approaches to the drug sensitivity problem in the literature it is highly desirable to compare these methods. Directly comparing the results from the papers is however not feasible for several reasons. First, the papers report the performance of their models using different evaluation metrics such as Pearson correlation or accuracy. Second, while some papers aim to predict IC50, others focus on the area under the dose-response curve, or the slope of the curve at some point. Also several papers use a binarized version of these metrics, reflecting "sensitive" versus "resistant", and the thresholds can vary. Third, different datasets are available: the GDSC and CCLE are most commonly used, but also the NCI60, the CGP, the CTRP and in-house datasets are used. Some works use a single dataset for training, validation and testing, while others use one dataset for training and hyperparameter tuning and use an independent dataset for validation. This brings us to the fourth difference: several data splits are used, e.g. some use a cross validation strategy whereas others use a single split. Finally, some papers use a multi-task approach while others use a single-task (i.e. drug) approach.

Two studies compared a wide range of methods for the drug sensitivity prediction problem. Costello et al. [2014] describes the results of the NCI DREAM drug sensitivity prediction challenge. The challengers provided datasets containing genomic, proteomic and epigenomic profiling data from 35 breast cancer cell lines, together with their sensitivity to 28 drug compounds. Participants were asked to provide a methodology to rank the cell lines according to their sensitivity for each drug, which was then tested on 18 unseen cell lines. The predictive performance of 44 participating teams was compared, and a kernelized regression approach outperformed the others. Additionally, the authors assessed the performance of an aggregated prediction from the 44 submitted approaches. This approach outperformed all individual methods, implying that the approaches provided non-overlapping information. Gene expression was found to be the most important predictor. Jang et al. [2014] systematically compare a variety of combinations of algorithms, types of molecular cell line characteristics, compounds and response metric (both continuous and discretized). The authors conclude that gene expression is the most informative molecular feature type, and elastic net and ridge regression generally outperform LASSO, RF, SVM, principal component regression (PCR) and partial least squares (PLS).

# References

Jordi Barretina, Giordano Caponigro, Nicolas Stransky, Kavitha Venkatesan, Adam A Margolin, Sungjoon Kim, Christopher J Wilson, Joseph Lehár, Gregory V Kryukov, Dmitriy Sonkin, et al. The cancer cell line encyclopedia enables predictive modelling of anticancer drug sensitivity. *Nature*, 483(7391):603, 2012.

Ting-Huei Chen and Wei Sun. Prediction of cancer drug sensitivity using high-dimensional omic features. *Biostatistics*, 18(1):1–14, 2017.

Isidro Cortés-Ciriano, Gerard JP van Westen, Guillaume Bouvier, Michael Nilges, John P Overington, Andreas Bender, and Thérèse E Malliavin. Improved large-scale prediction of growth inhibition patterns using the nci60 cancer cell line panel. *Bioinformatics*, 32(1):85–95, 2015.

James C Costello, Laura M Heiser, Elisabeth Georgii, Mehmet Gönen, Michael P Menden, Nicholas J Wang, Mukesh Bansal, Petteri Hintsanen, Suleiman A Khan, John-Patrick Mpindi, et al. A community effort to assess and improve drug sensitivity prediction algorithms. *Nature biotechnology*, 32(12):1202, 2014.

Zuoli Dong, Naiqian Zhang, Chun Li, Haiyun Wang, Yun Fang, Jun Wang, and Xiaoqi Zheng. Anticancer drug sensitivity prediction in cell lines from baseline gene expression through recursive feature selection. *BMC cancer*, 15(1):489, 2015.

Mathew J Garnett, Elena J Edelman, Sonja J Heidorn, Chris D Greenman, Anahita Dastur, King Wai Lau, Patricia Greninger, I Richard Thompson, Xi Luo, Jorge Soares, et al. Systematic identification of genomic markers of drug sensitivity in cancer cells. *Nature*, 483(7391):570, 2012.

Mehmet Gönen and Adam A Margolin. Drug susceptibility prediction against a panel of drugs using kernelized bayesian multitask learning. *Bioinformatics*, 30(17):i556–i563, 2014.

Jochen Graw. *Genetik*. Springer, 2015.

Sudheer Gupta, Kumardeep Chaudhary, Rahul Kumar, Ankur Gautam, Jagpreet Singh Nanda, Sandeep Kumar Dhanda, Samir Kumar Brahmachari, and Gajendra PS Raghava. Prioritization of anticancer drugs against a cancer using genomic features of cancer cells: A step towards personalized medicine. *Scientific reports*, 6:23857, 2016.

Francesco Iorio, Theo A Knijnenburg, Daniel J Vis, Graham R Bignell, Michael P Menden, Michael Schubert, Nanne Aben, Emanuel Gonçalves, Syd Barthorpe, Howard Lightfoot, et al. A landscape of pharmacogenomic interactions in cancer. *Cell*, 166(3):740–754, 2016.

In Sock Jang, Elias Chaibub Neto, Justin Guinney, Stephen H Friend, and Adam A Margolin. Systematic assessment of analytical methods for drug sensitivity prediction from cancer cell line data. In *Biocomputing 2014*, pages 63–74. World Scientific, 2014.

Jouhyun Jeon, Satra Nim, Joan Teyra, Alessandro Datti, Jeffrey L Wrana, Sachdev S Sidhu, Jason Moffat, and Philip M Kim. A systematic approach to identify novel cancer drug targets using machine learning, inhibitor design and high-throughput screening. *Genome medicine*, 6(7):57, 2014.

Michael P Menden, Francesco Iorio, Mathew Garnett, Ultan McDermott, Cyril H Benes, Pedro J Ballester, and Julio Saez-Rodriguez. Machine learning prediction of cancer cell sensitivity to drugs based on genomic and chemical properties. *PLoS one*, 8(4):e61318, 2013.

Simon Papillon-Cavanagh, Nicolas De Jay, Nehme Hachem, Catharina Olsen, Gianluca Bontempi, Hugo JWL Aerts, John Quackenbush, and Benjamin Haibe-Kains. Comparison and validation of genomic predictors for anticancer drug sensitivity. *Journal of the American Medical Informatics Association*, 20(4):597–602, 2013.

Daniel R Rhodes, Jianjun Yu, K Shanker, Nandan Deshpande, Radhika Varambally, Debashis Ghosh, Terrence Barrette, Akhilesh Pandey, and Arul M Chinnaiyan. Large-scale meta-analysis of cancer microarray data identifies common transcriptional profiles of neoplastic transformation and progression. *Proceedings of the National Academy of Sciences*, 101(25):9309–9314, 2004.

Olaf Schmidt. *Genetik und Molekularbiologie*. Springer, 2017.

Chayaporn Suphavilai, Denis Bertrand, and Niranjan Nagarajan. Predicting cancer drug response using a recommender system. *Bioinformatics*, 34:3907–3914, 2018.

Mehmet Tan. Prediction of anti-cancer drug response by kernelized multi-task learning. *Artificial intelligence in medicine*, 73:70–77, 2016.

Xuewei Wang, Zhifu Sun, Michael T Zimmermann, Andrej Bugrim, and Jean-Pierre Kocher. Predict drug sensitivity of cancer cells with pathway activity inference. *BMC medical genomics*, 12(1):15, 2019.

Qinghua Xu, Jinying Chen, Shujuan Ni, Cong Tan, Midie Xu, Lei Dong, Lin Yuan, Qifeng Wang, and Xiang Du. Pan-cancer transcriptome analysis reveals a gene expression signature for the identification of tumor tissue origin. *Modern Pathology*, 29(6):546, 2016.

Mi Yang, Jaak Simm, Chi Chung Lam, Pooya Zakeri, Gerard JP van Westen, Yves Moreau, and Julio Saez-Rodriguez. Linking drug target and pathway activation for effective therapy using multi-task learning. *Scientific reports*, 8, 2018.

Wanjuan Yang, Jorge Soares, Patricia Greninger, Elena J Edelman, Howard Lightfoot, Simon Forbes, Nidhi Bindal, Dave Beare, James A Smith, I Richard Thompson, et al. Genomics of drug sensitivity in cancer (GDSC): a resource for therapeutic biomarker discovery in cancer cells. *Nucleic acids research*, 41(D1):D955–D961, 2013.

Lin Zhang, Xing Chen, Na-Na Guan, Hui Liu, and Jian-Qiang Li. A hybrid interpolation weighted collaborative filtering method for anti-cancer drug response prediction. *Frontiers in Pharmacology*, 9, 2018.
